# Supplementary material for: Learning Compact Recurrent Neural Networks with Block-Term Tensor Decomposition
Source: arXiv:1712.05134 source file (2018-05-11)
Supplement: Supplementary file 1 [file supplement.tex]

\begin{figure*}[t]
    \centering
    \subfigure[][block1,factor2]{\includegraphics[height=0.45\columnwidth]{experiments/img_gen/GRU/type1_rank1_block1_factors2_9} } \quad
    \subfigure[][block1,factor3]{\includegraphics[height=0.45\columnwidth]{experiments/img_gen/GRU/type1_rank1_block1_factors3_9} } \quad
    \subfigure[][block1,factor4]{\includegraphics[height=0.45\columnwidth]{experiments/img_gen/GRU/type1_rank1_block1_factors4_9} } \quad
    \subfigure[][block1,factor5]{\includegraphics[height=0.45\columnwidth]{experiments/img_gen/GRU/type1_rank1_block1_factors5_9} } \quad \\
    
    \subfigure[][block2,factor2]{\includegraphics[height=0.45\columnwidth]{experiments/img_gen/GRU/type1_rank1_block2_factors2_9} } \quad
    \subfigure[][block2,factor3]{\includegraphics[height=0.45\columnwidth]{experiments/img_gen/GRU/type1_rank1_block2_factors3_9} } \quad
    \subfigure[][block2,factor4]{\includegraphics[height=0.45\columnwidth]{experiments/img_gen/GRU/type1_rank1_block2_factors4_9} } \quad
    \subfigure[][block2,factor5]{\includegraphics[height=0.45\columnwidth]{experiments/img_gen/GRU/type1_rank1_block2_factors5_9} } \quad \\
    
    \subfigure[][block3,factor2]{\includegraphics[height=0.45\columnwidth]{experiments/img_gen/GRU/type1_rank1_block3_factors2_9} } \quad
    \subfigure[][block3,factor3]{\includegraphics[height=0.45\columnwidth]{experiments/img_gen/GRU/type1_rank1_block3_factors3_9} } \quad
    \subfigure[][block3,factor4]{\includegraphics[height=0.45\columnwidth]{experiments/img_gen/GRU/type1_rank1_block3_factors4_9} } \quad
    \subfigure[][block3,factor5]{\includegraphics[height=0.45\columnwidth]{experiments/img_gen/GRU/type1_rank1_block3_factors5_9} } \quad \\
    
    \subfigure[][block4,factor2]{\includegraphics[height=0.45\columnwidth]{experiments/img_gen/GRU/type1_rank1_block4_factors2_9} } \quad
    \subfigure[][block4,factor3]{\includegraphics[height=0.45\columnwidth]{experiments/img_gen/GRU/type1_rank1_block4_factors3_9} } \quad
    \subfigure[][block4,factor4]{\includegraphics[height=0.45\columnwidth]{experiments/img_gen/GRU/type1_rank1_block4_factors4_9} } \quad
    \subfigure[][block4,factor5]{\includegraphics[height=0.45\columnwidth]{experiments/img_gen/GRU/type1_rank1_block4_factors5_9} } \quad \\

    \caption{GRU, rank = 1, vary by block and factor. }
    \label{nonlinear_connections}
    \end{figure*}

    \newpage
    \null
    \newpage

    \begin{figure*}
        \centering 
        \subfigure[][Original, P=4096]{\includegraphics[height=0.3\columnwidth]{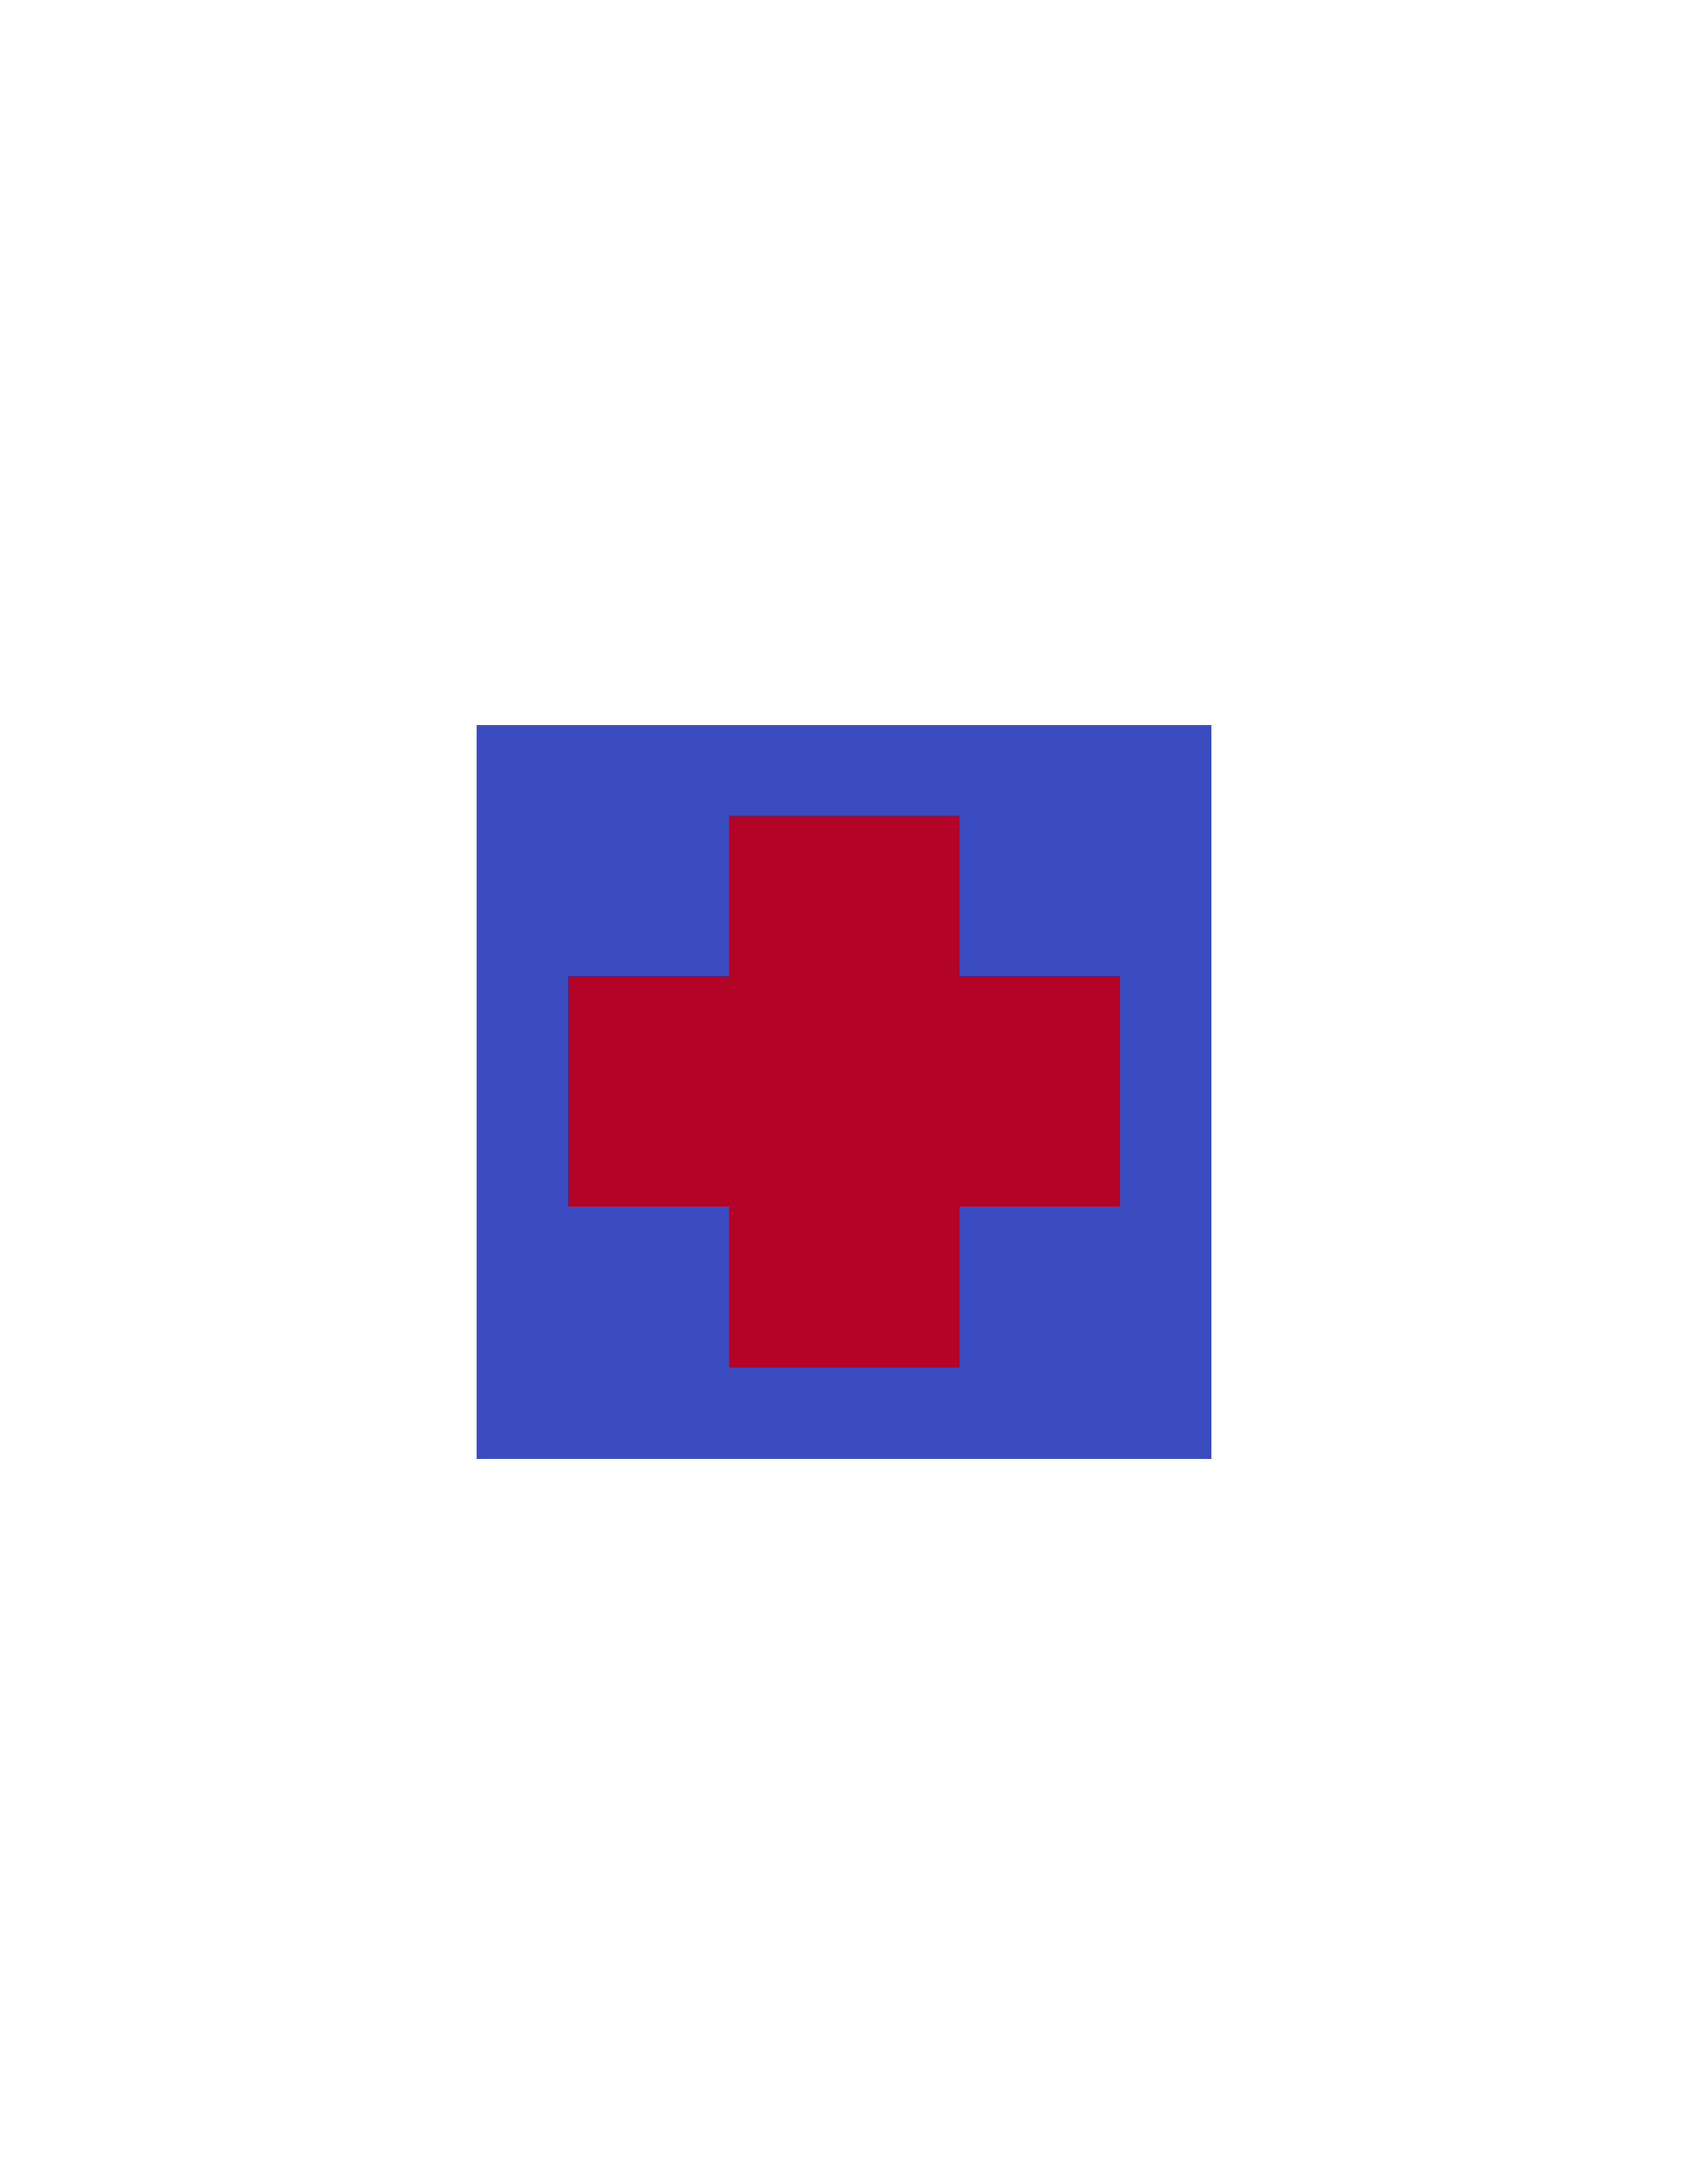}} \quad 
        \subfigure[][Linear Regression, P=4096]{\includegraphics[height=0.3\columnwidth]{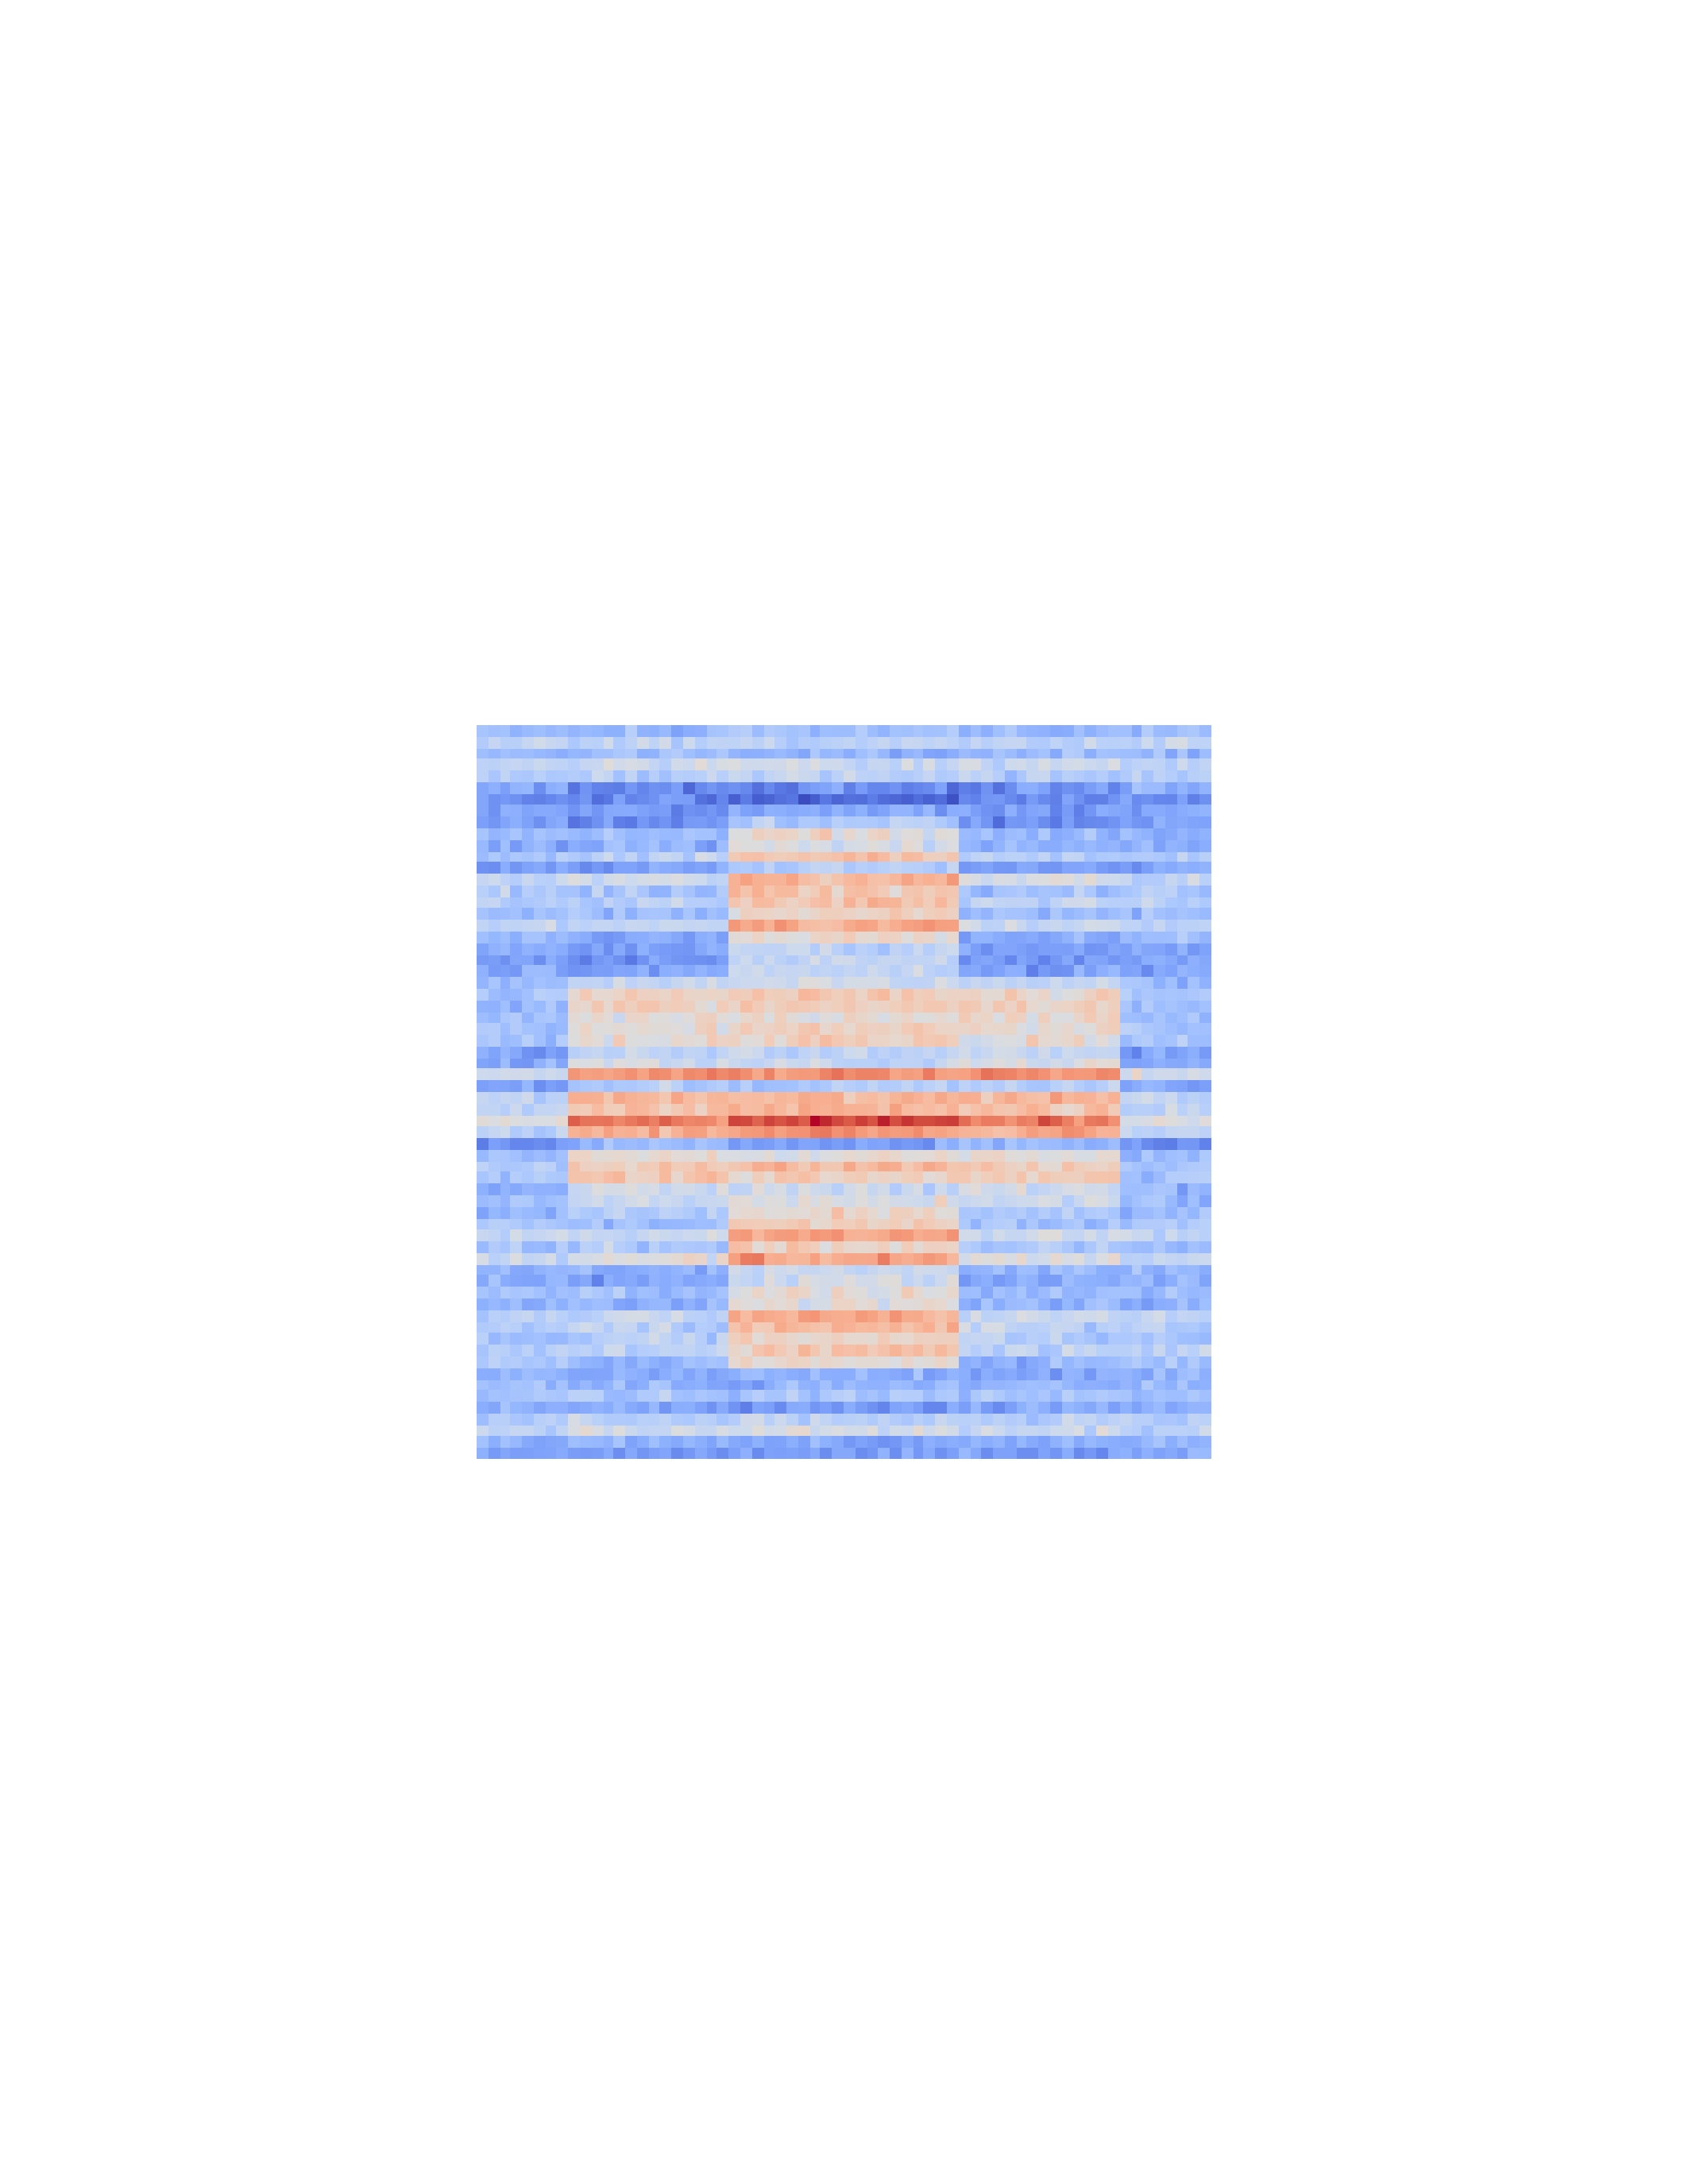}} \quad 
        \subfigure[][d=2,R=1,N=1,P=129]{\includegraphics[height=0.3\columnwidth]{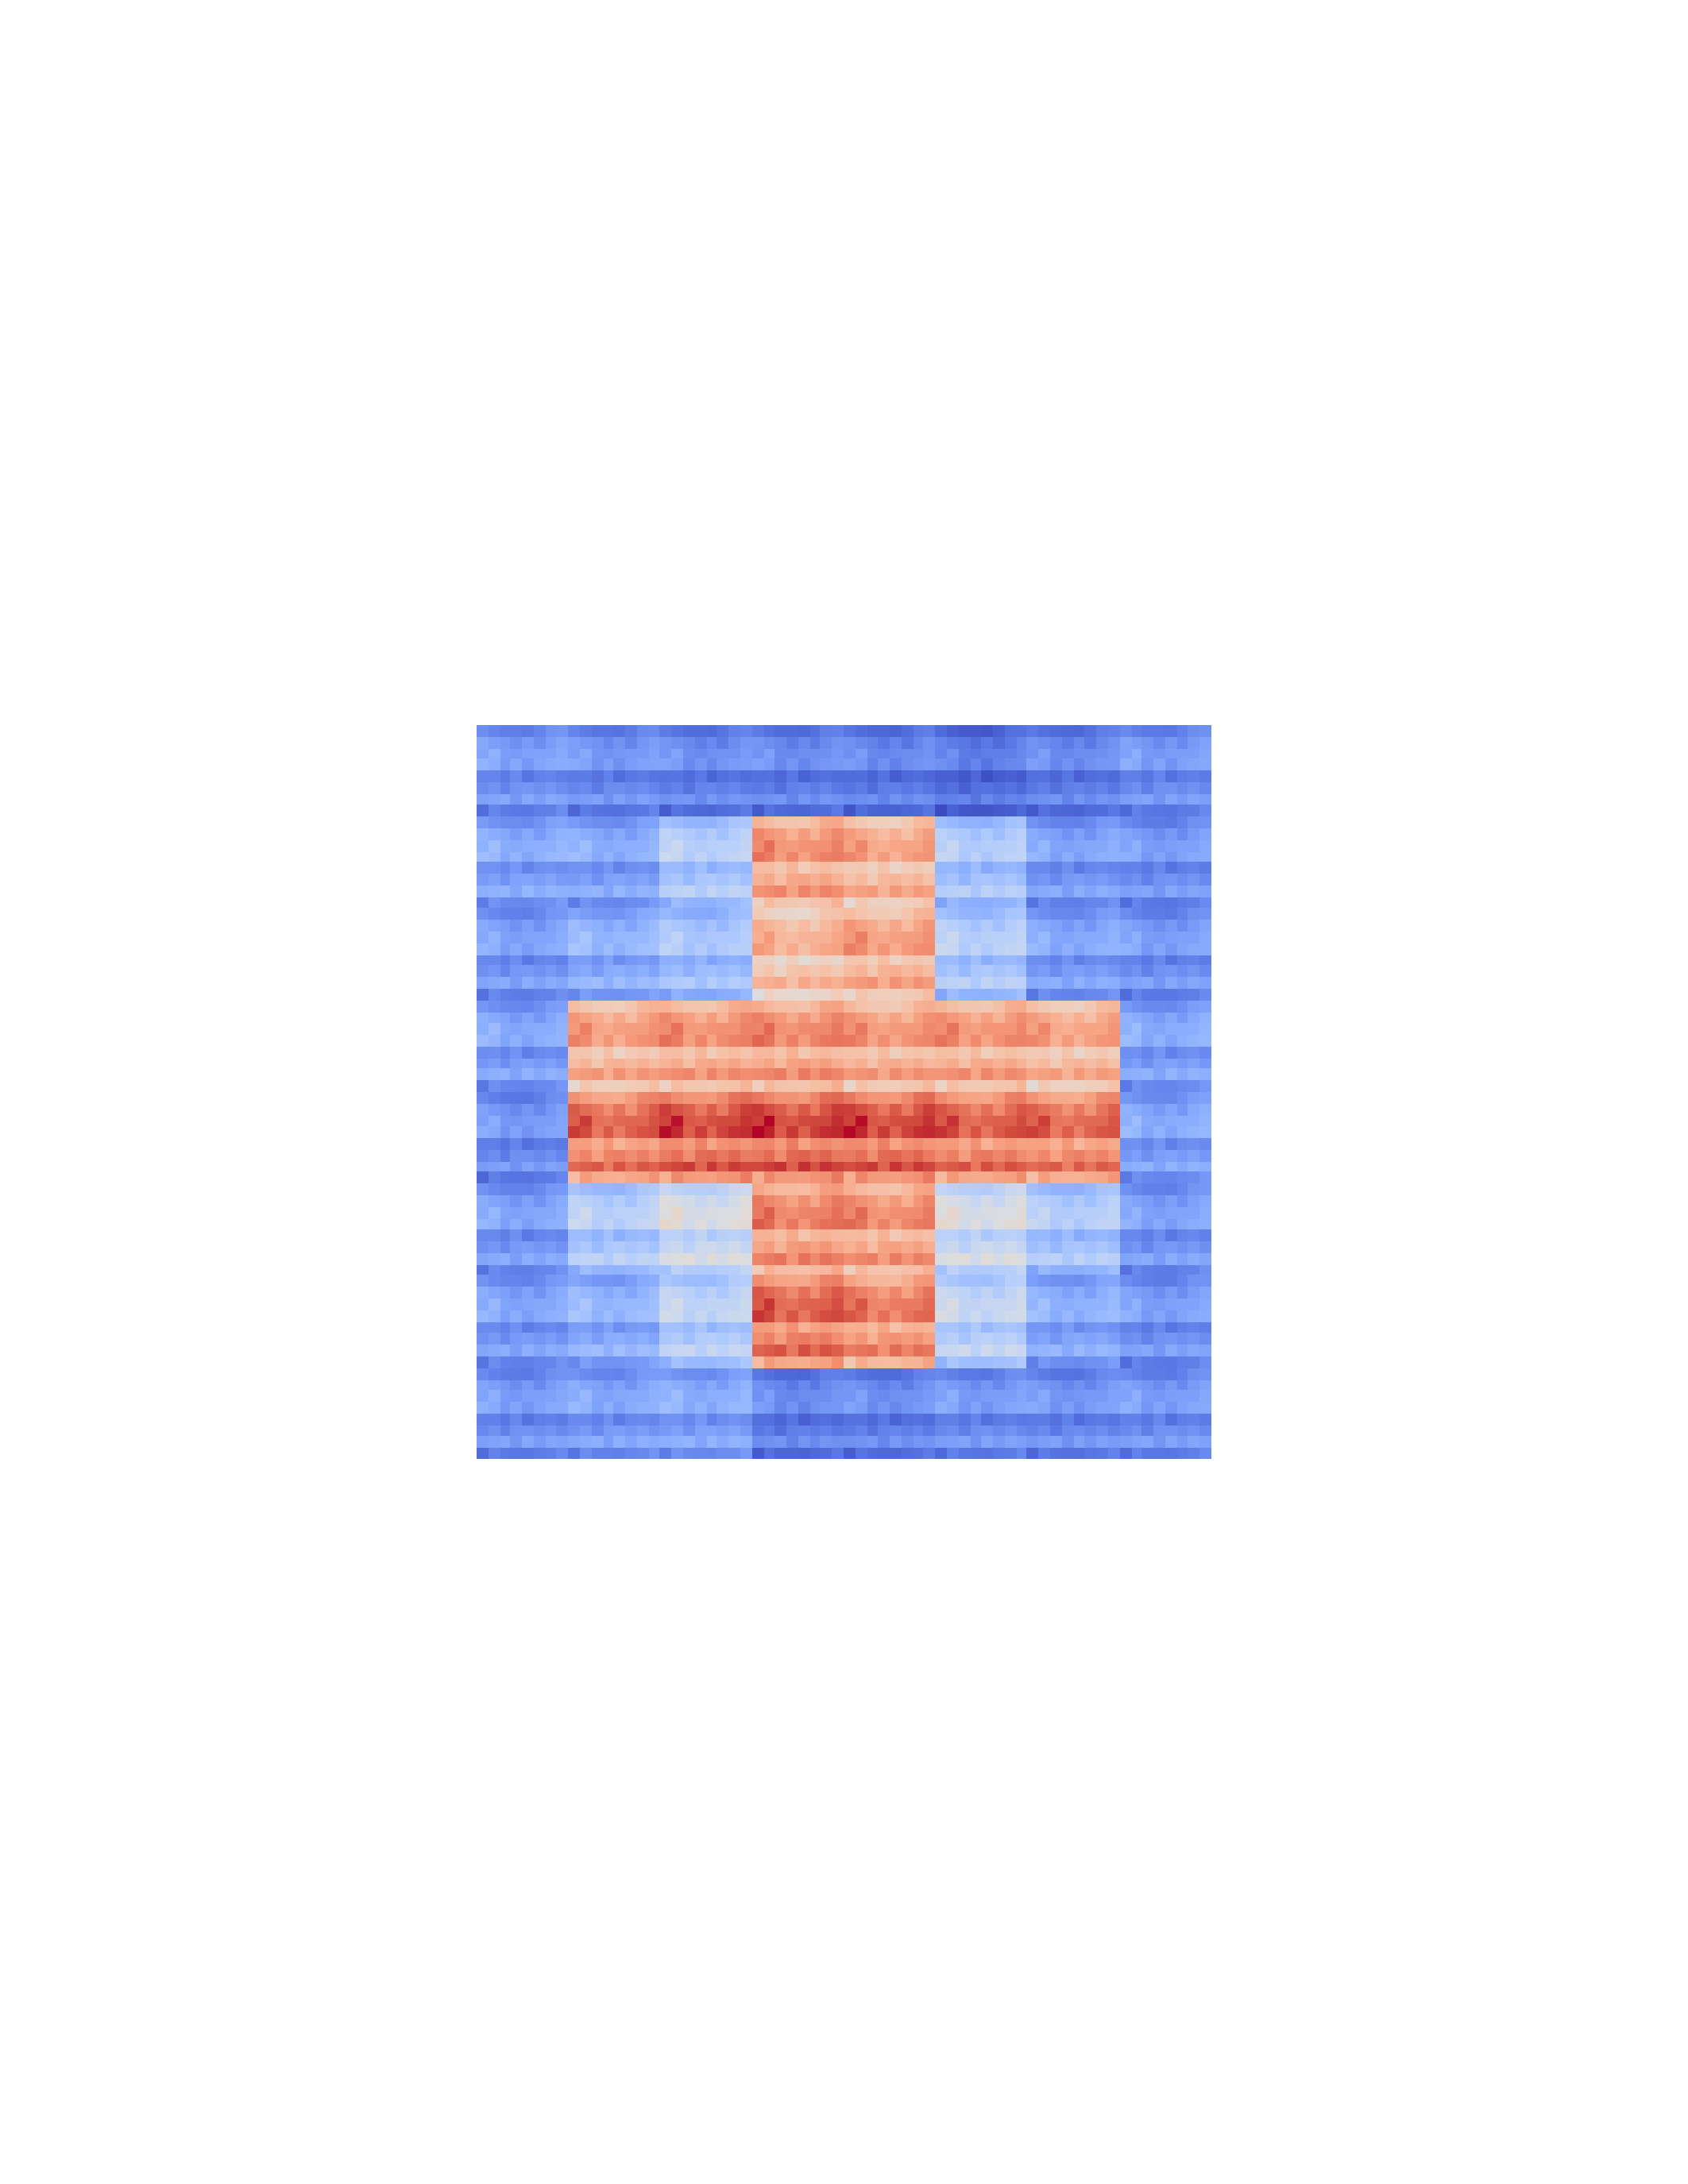}}  \quad 
        \subfigure[][d=2,R=2,N=1,P=260]{\includegraphics[height=0.3\columnwidth]{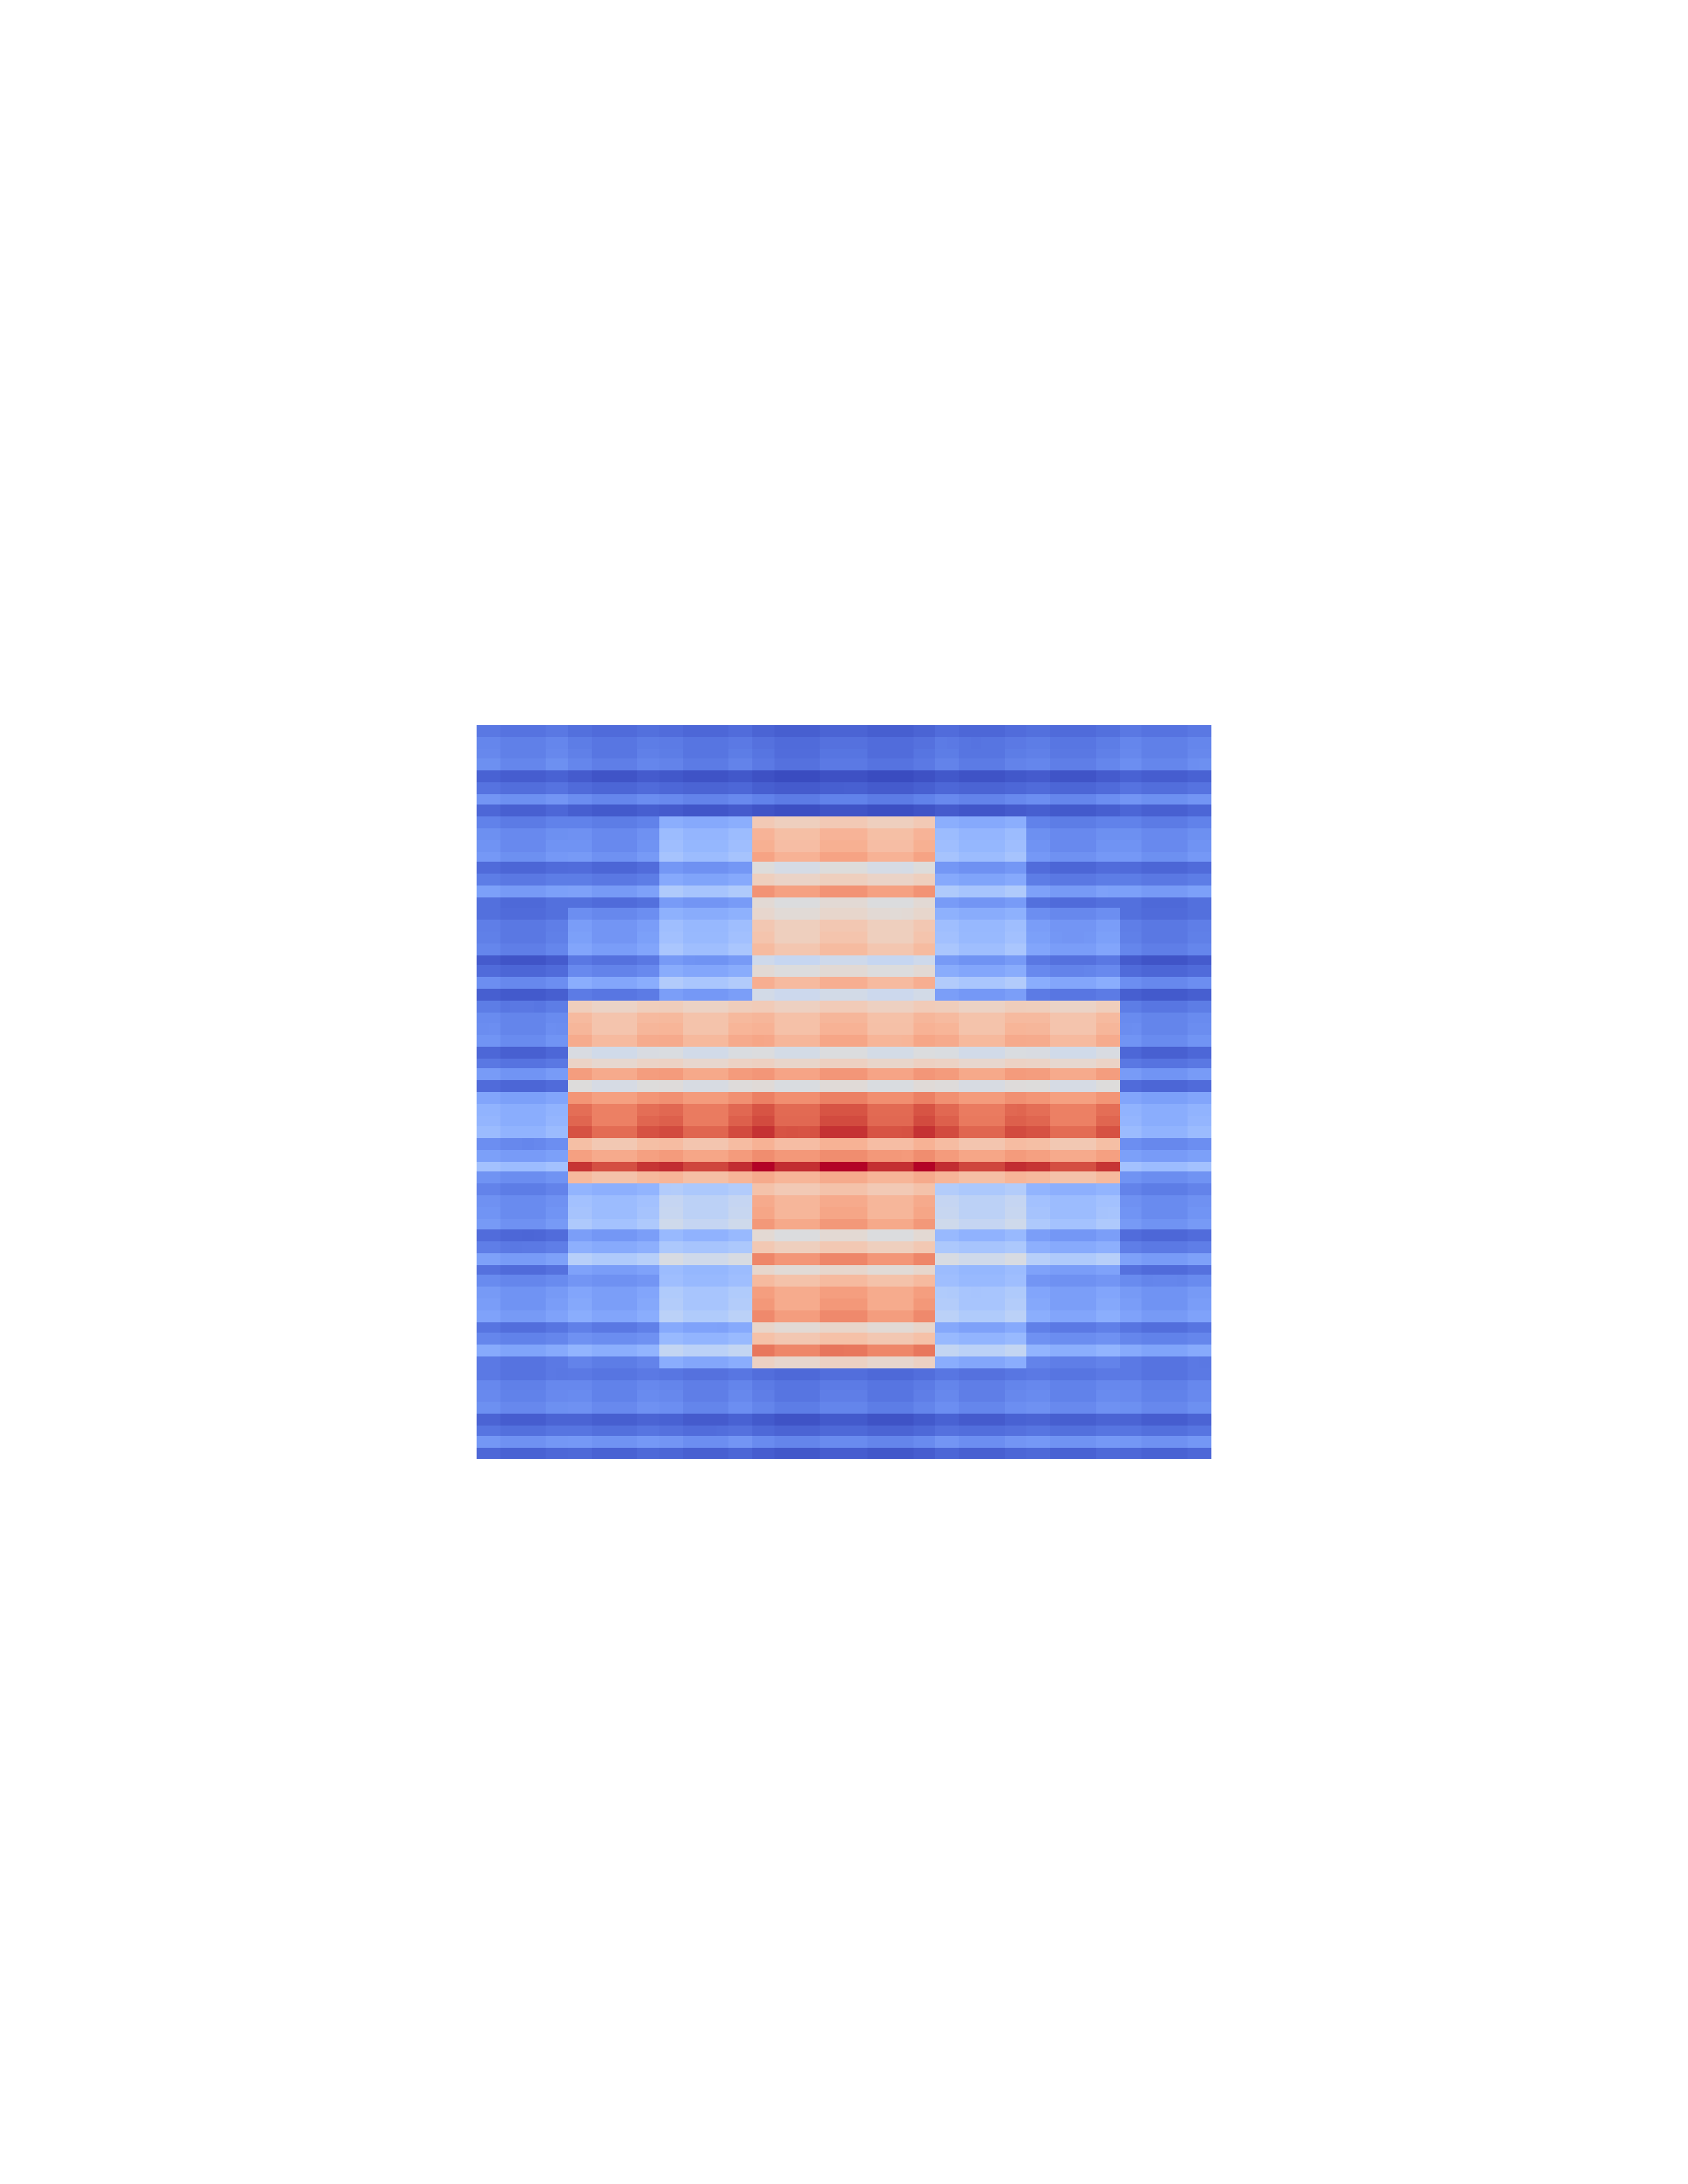}}  \quad 
        \subfigure[][d=2,R=3,N=1,P=393]{\includegraphics[height=0.3\columnwidth]{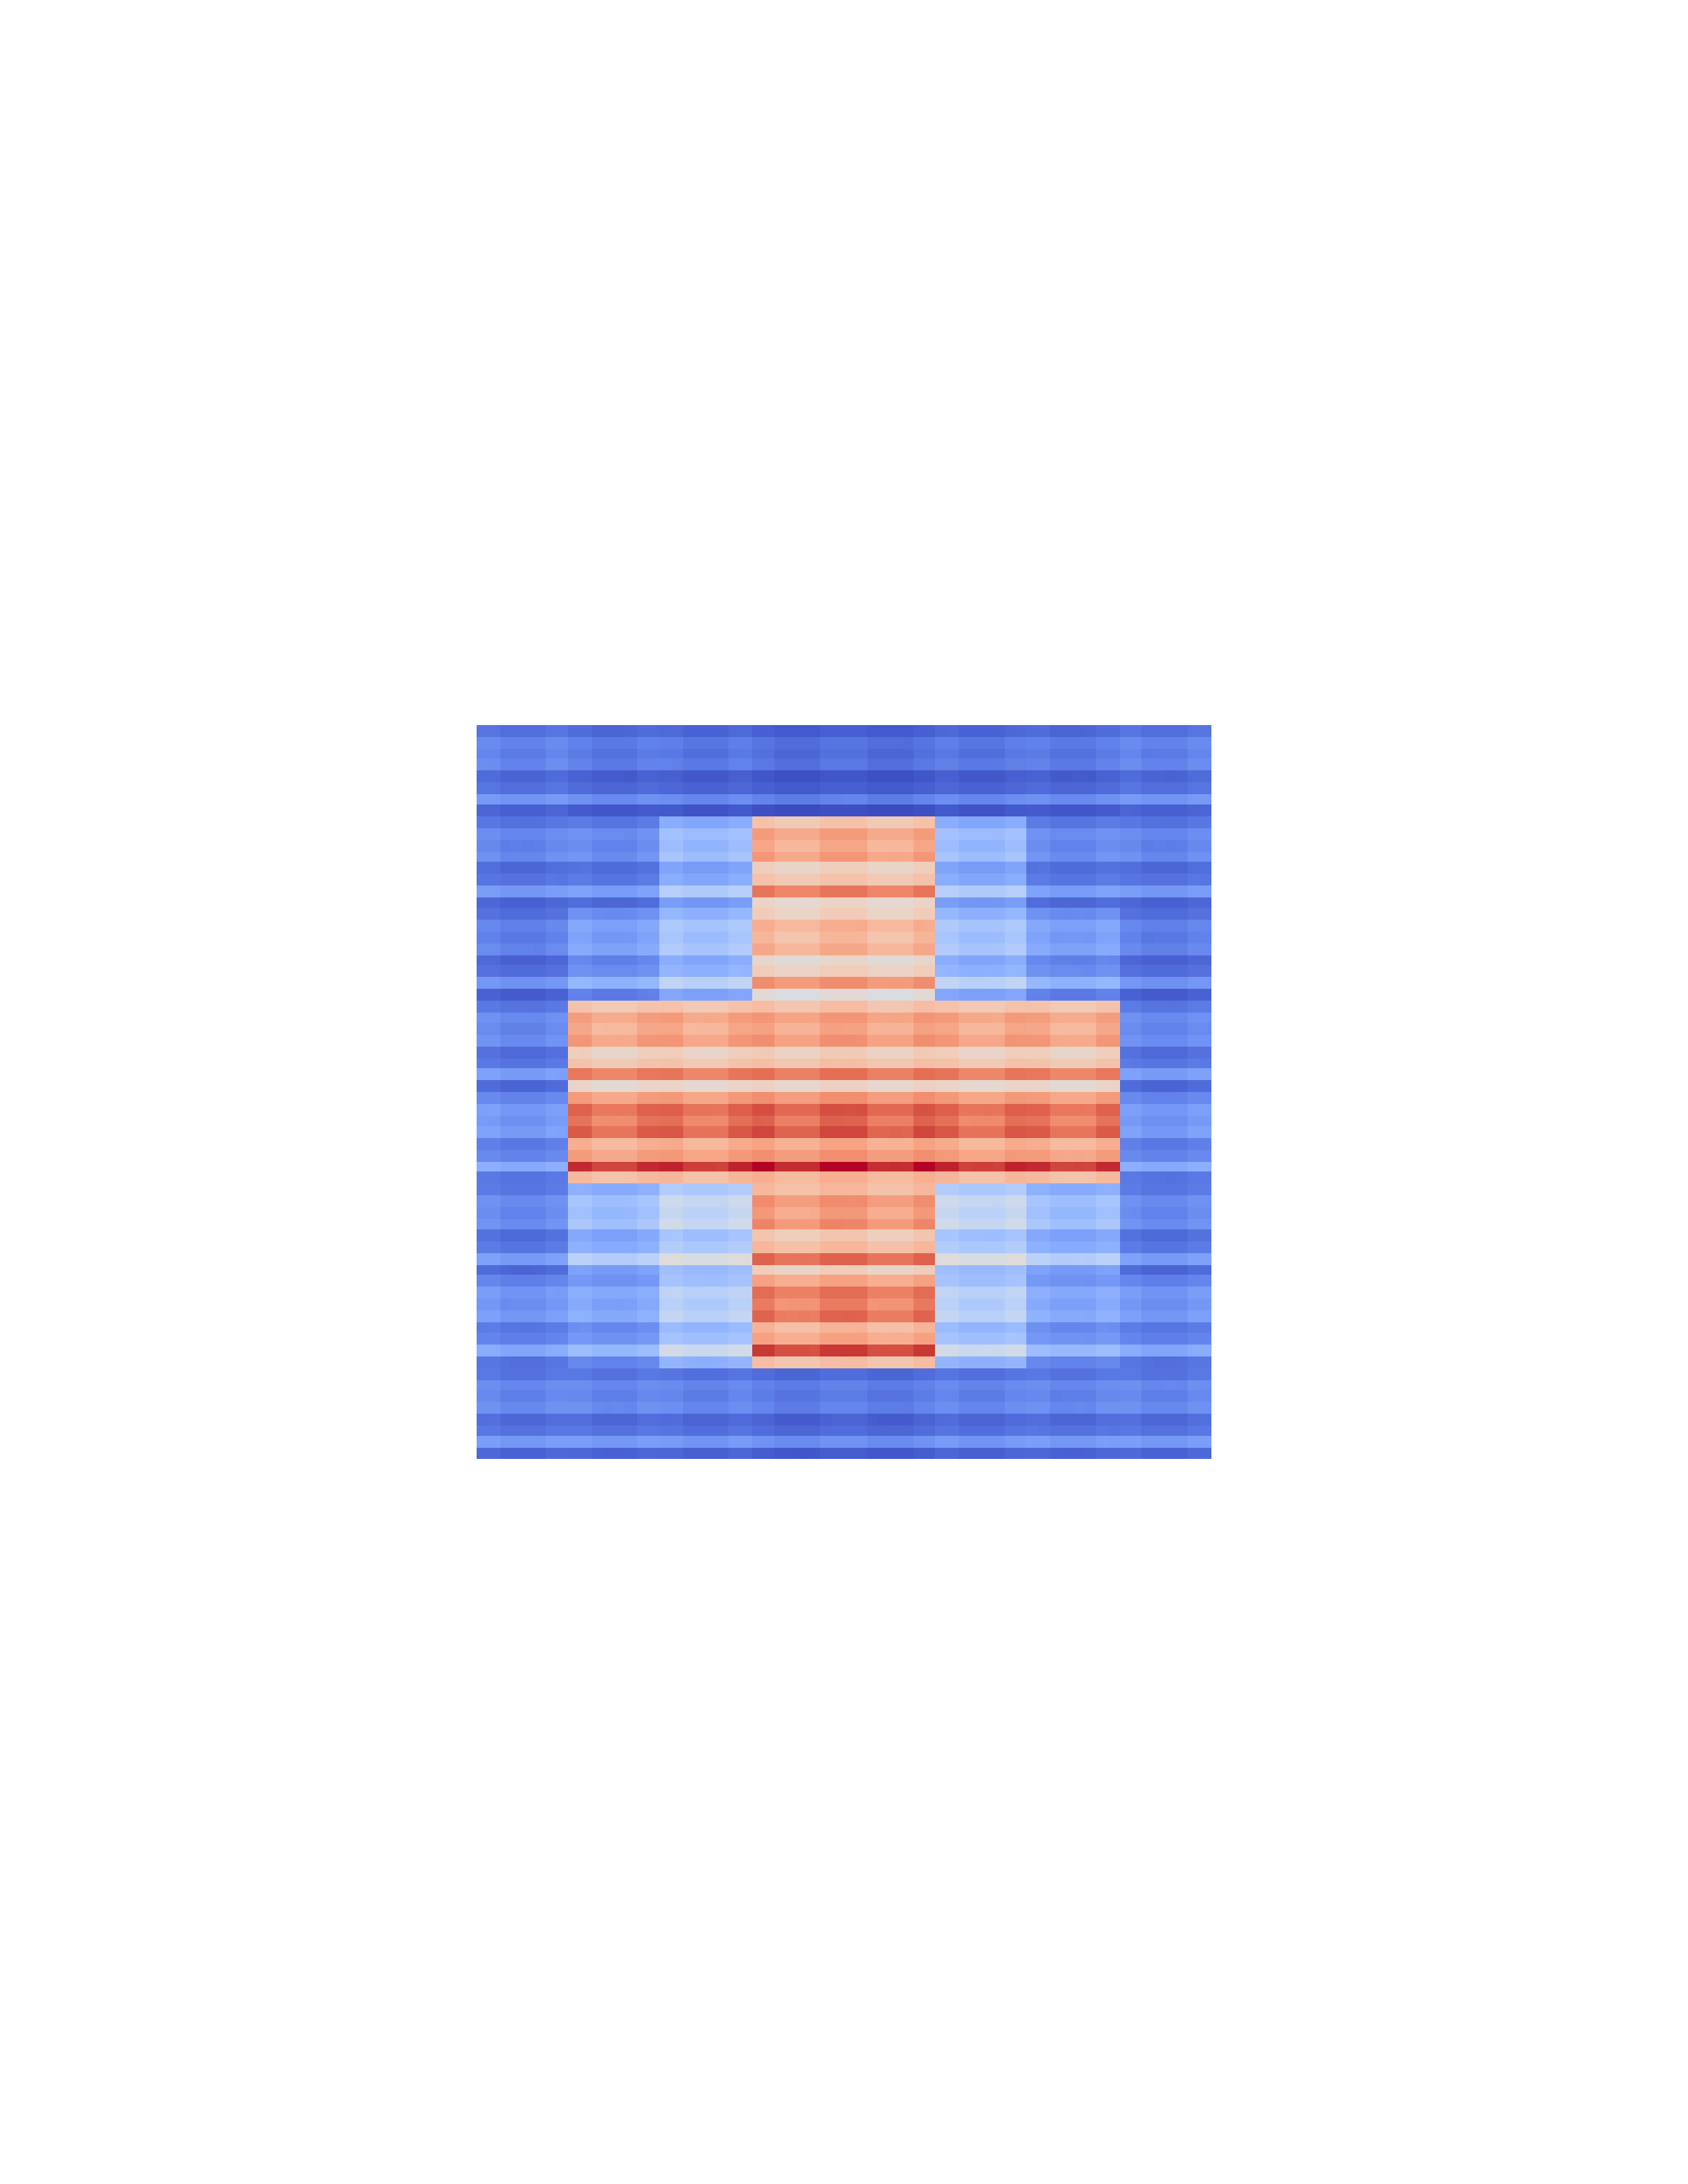}}  \quad 
        \subfigure[][d=2,R=4,N=1,P=528]{\includegraphics[height=0.3\columnwidth]{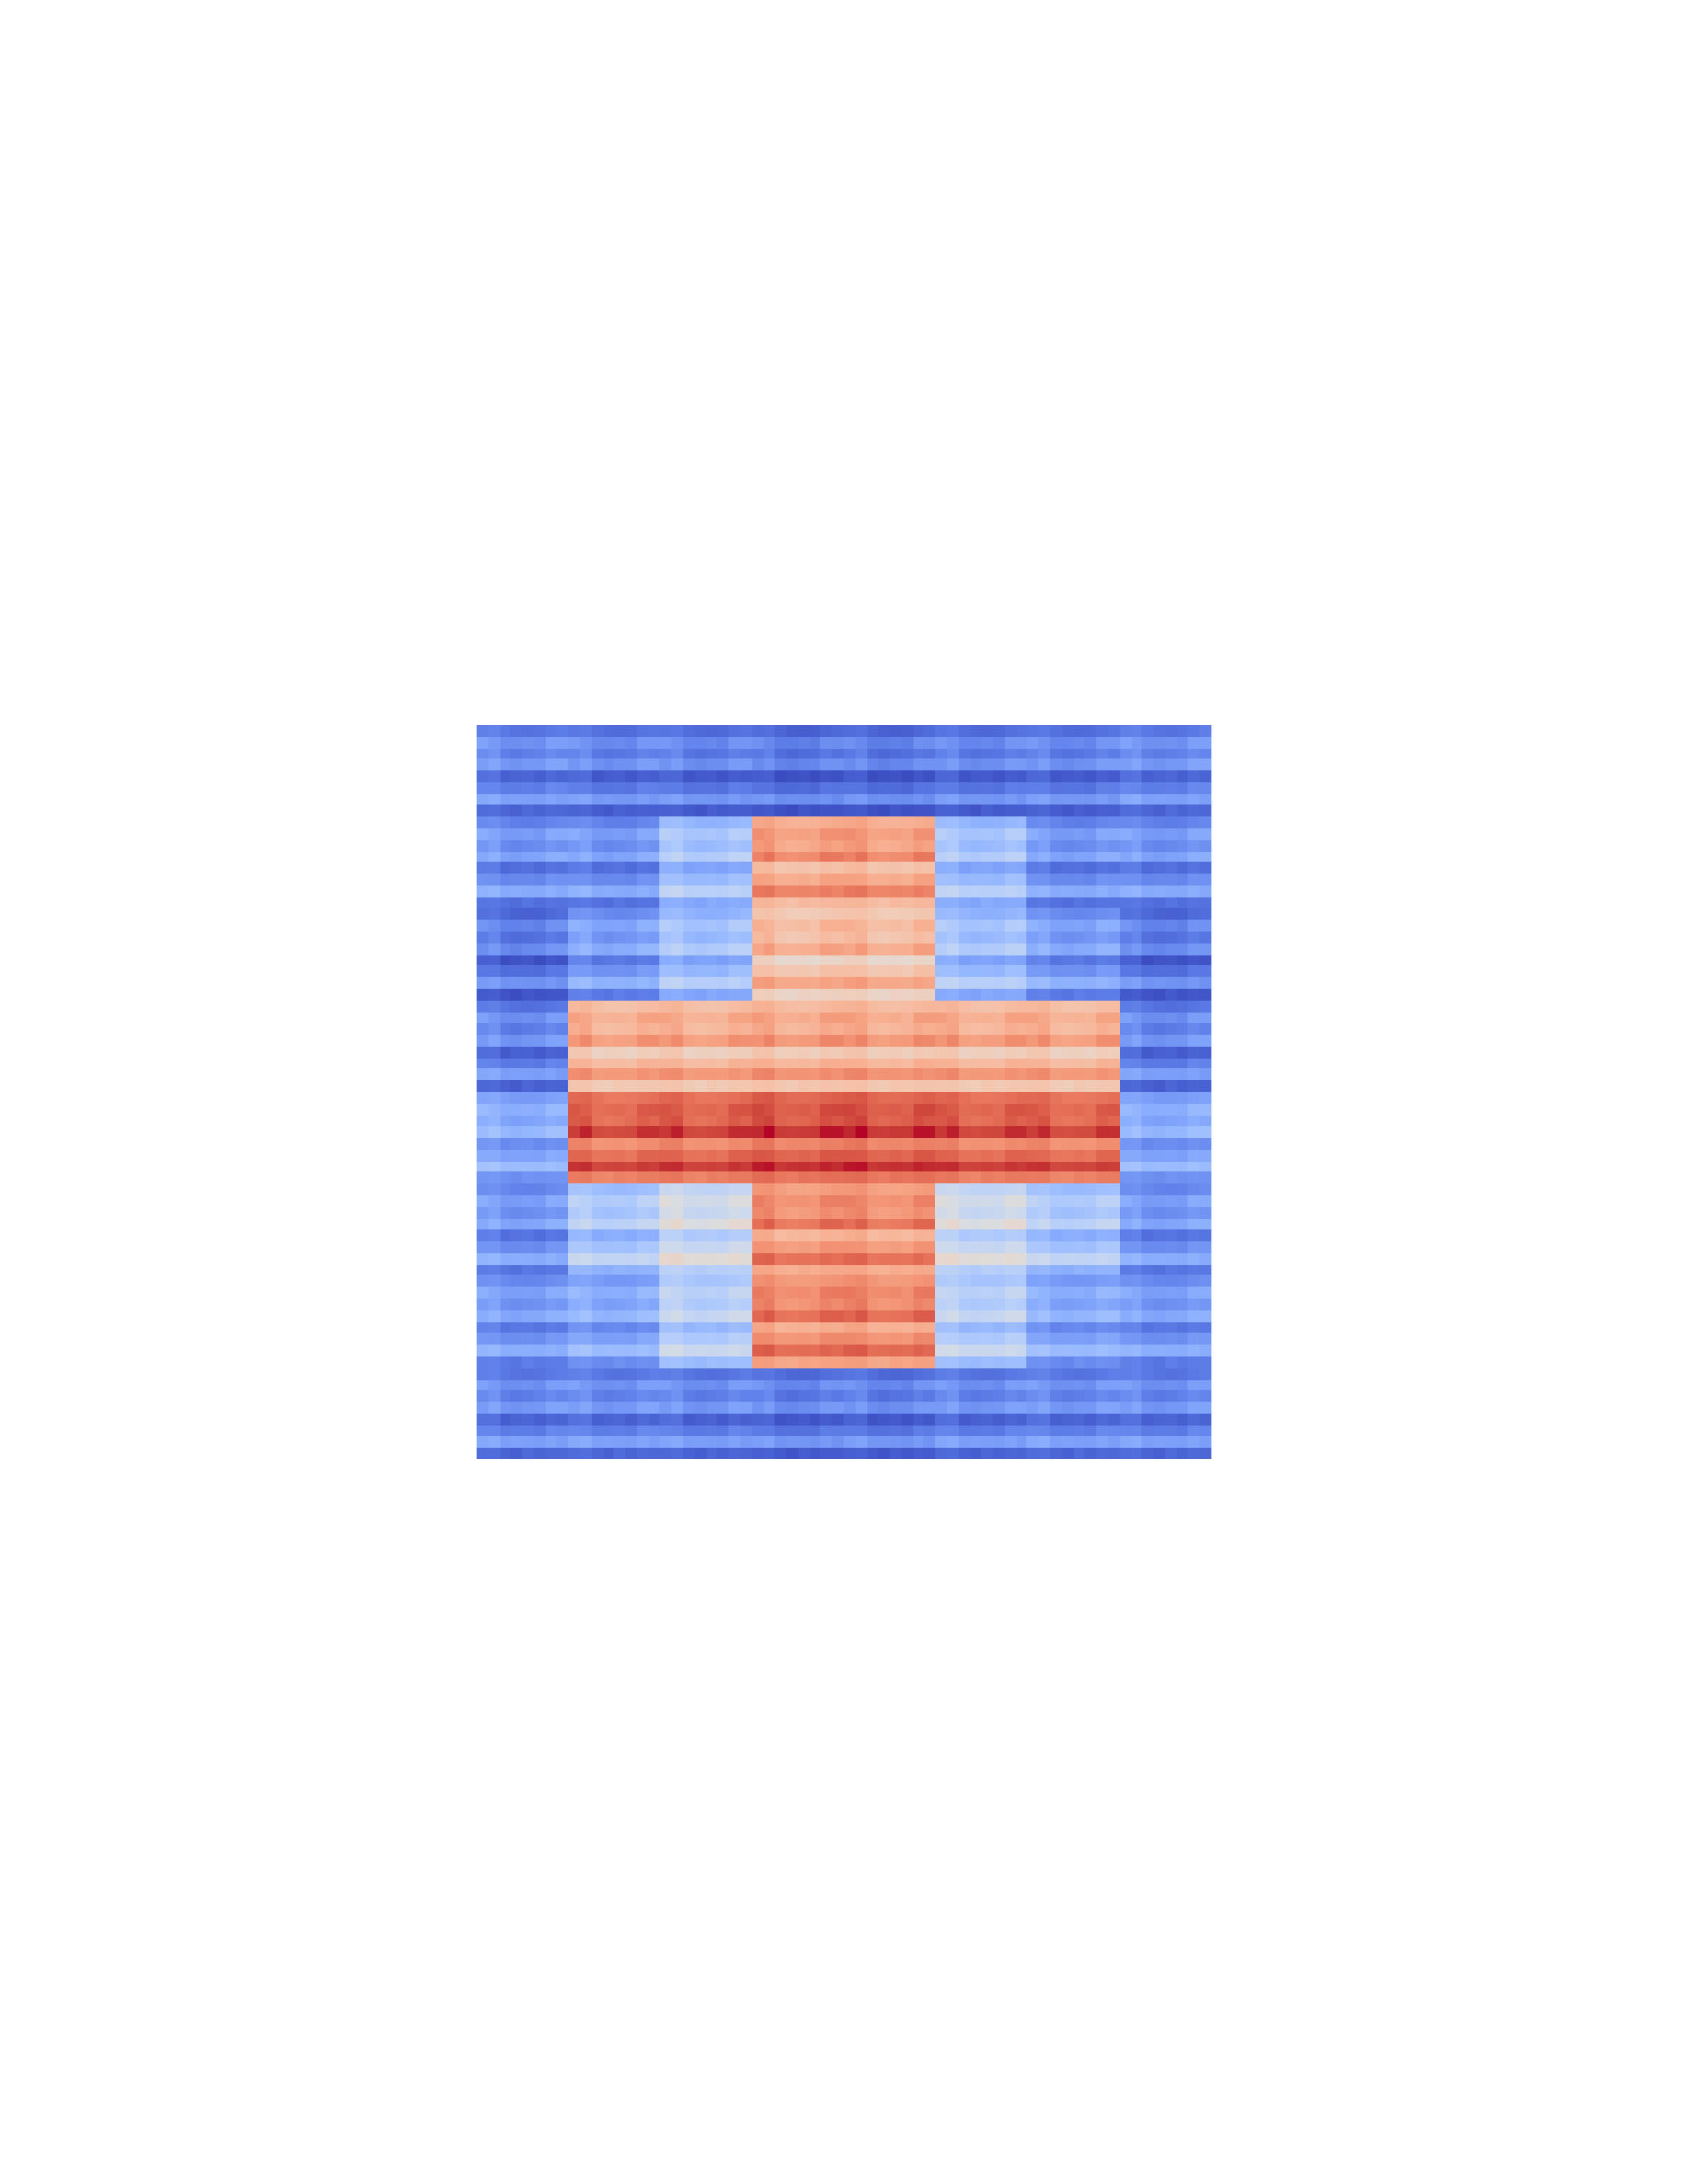}} 
        \caption{Rank variant.}
    \end{figure*}

    \begin{figure*}
        \centering 
        \subfigure[][Original, P=4096]{\includegraphics[height=0.3\columnwidth]{pics/synthetic/original_d2_b1.eps}} \quad 
        \subfigure[][Linear Regression, P=4096]{\includegraphics[height=0.3\columnwidth]{pics/synthetic/linear_d2_b1.eps}} \quad 
        \subfigure[][d=2,R=1,N=1,P=129]{\includegraphics[height=0.3\columnwidth]{pics/synthetic/d2_R1_N1.eps}}  \quad 
        \subfigure[][d=2,R=1,N=2,P=258]{\includegraphics[height=0.3\columnwidth]{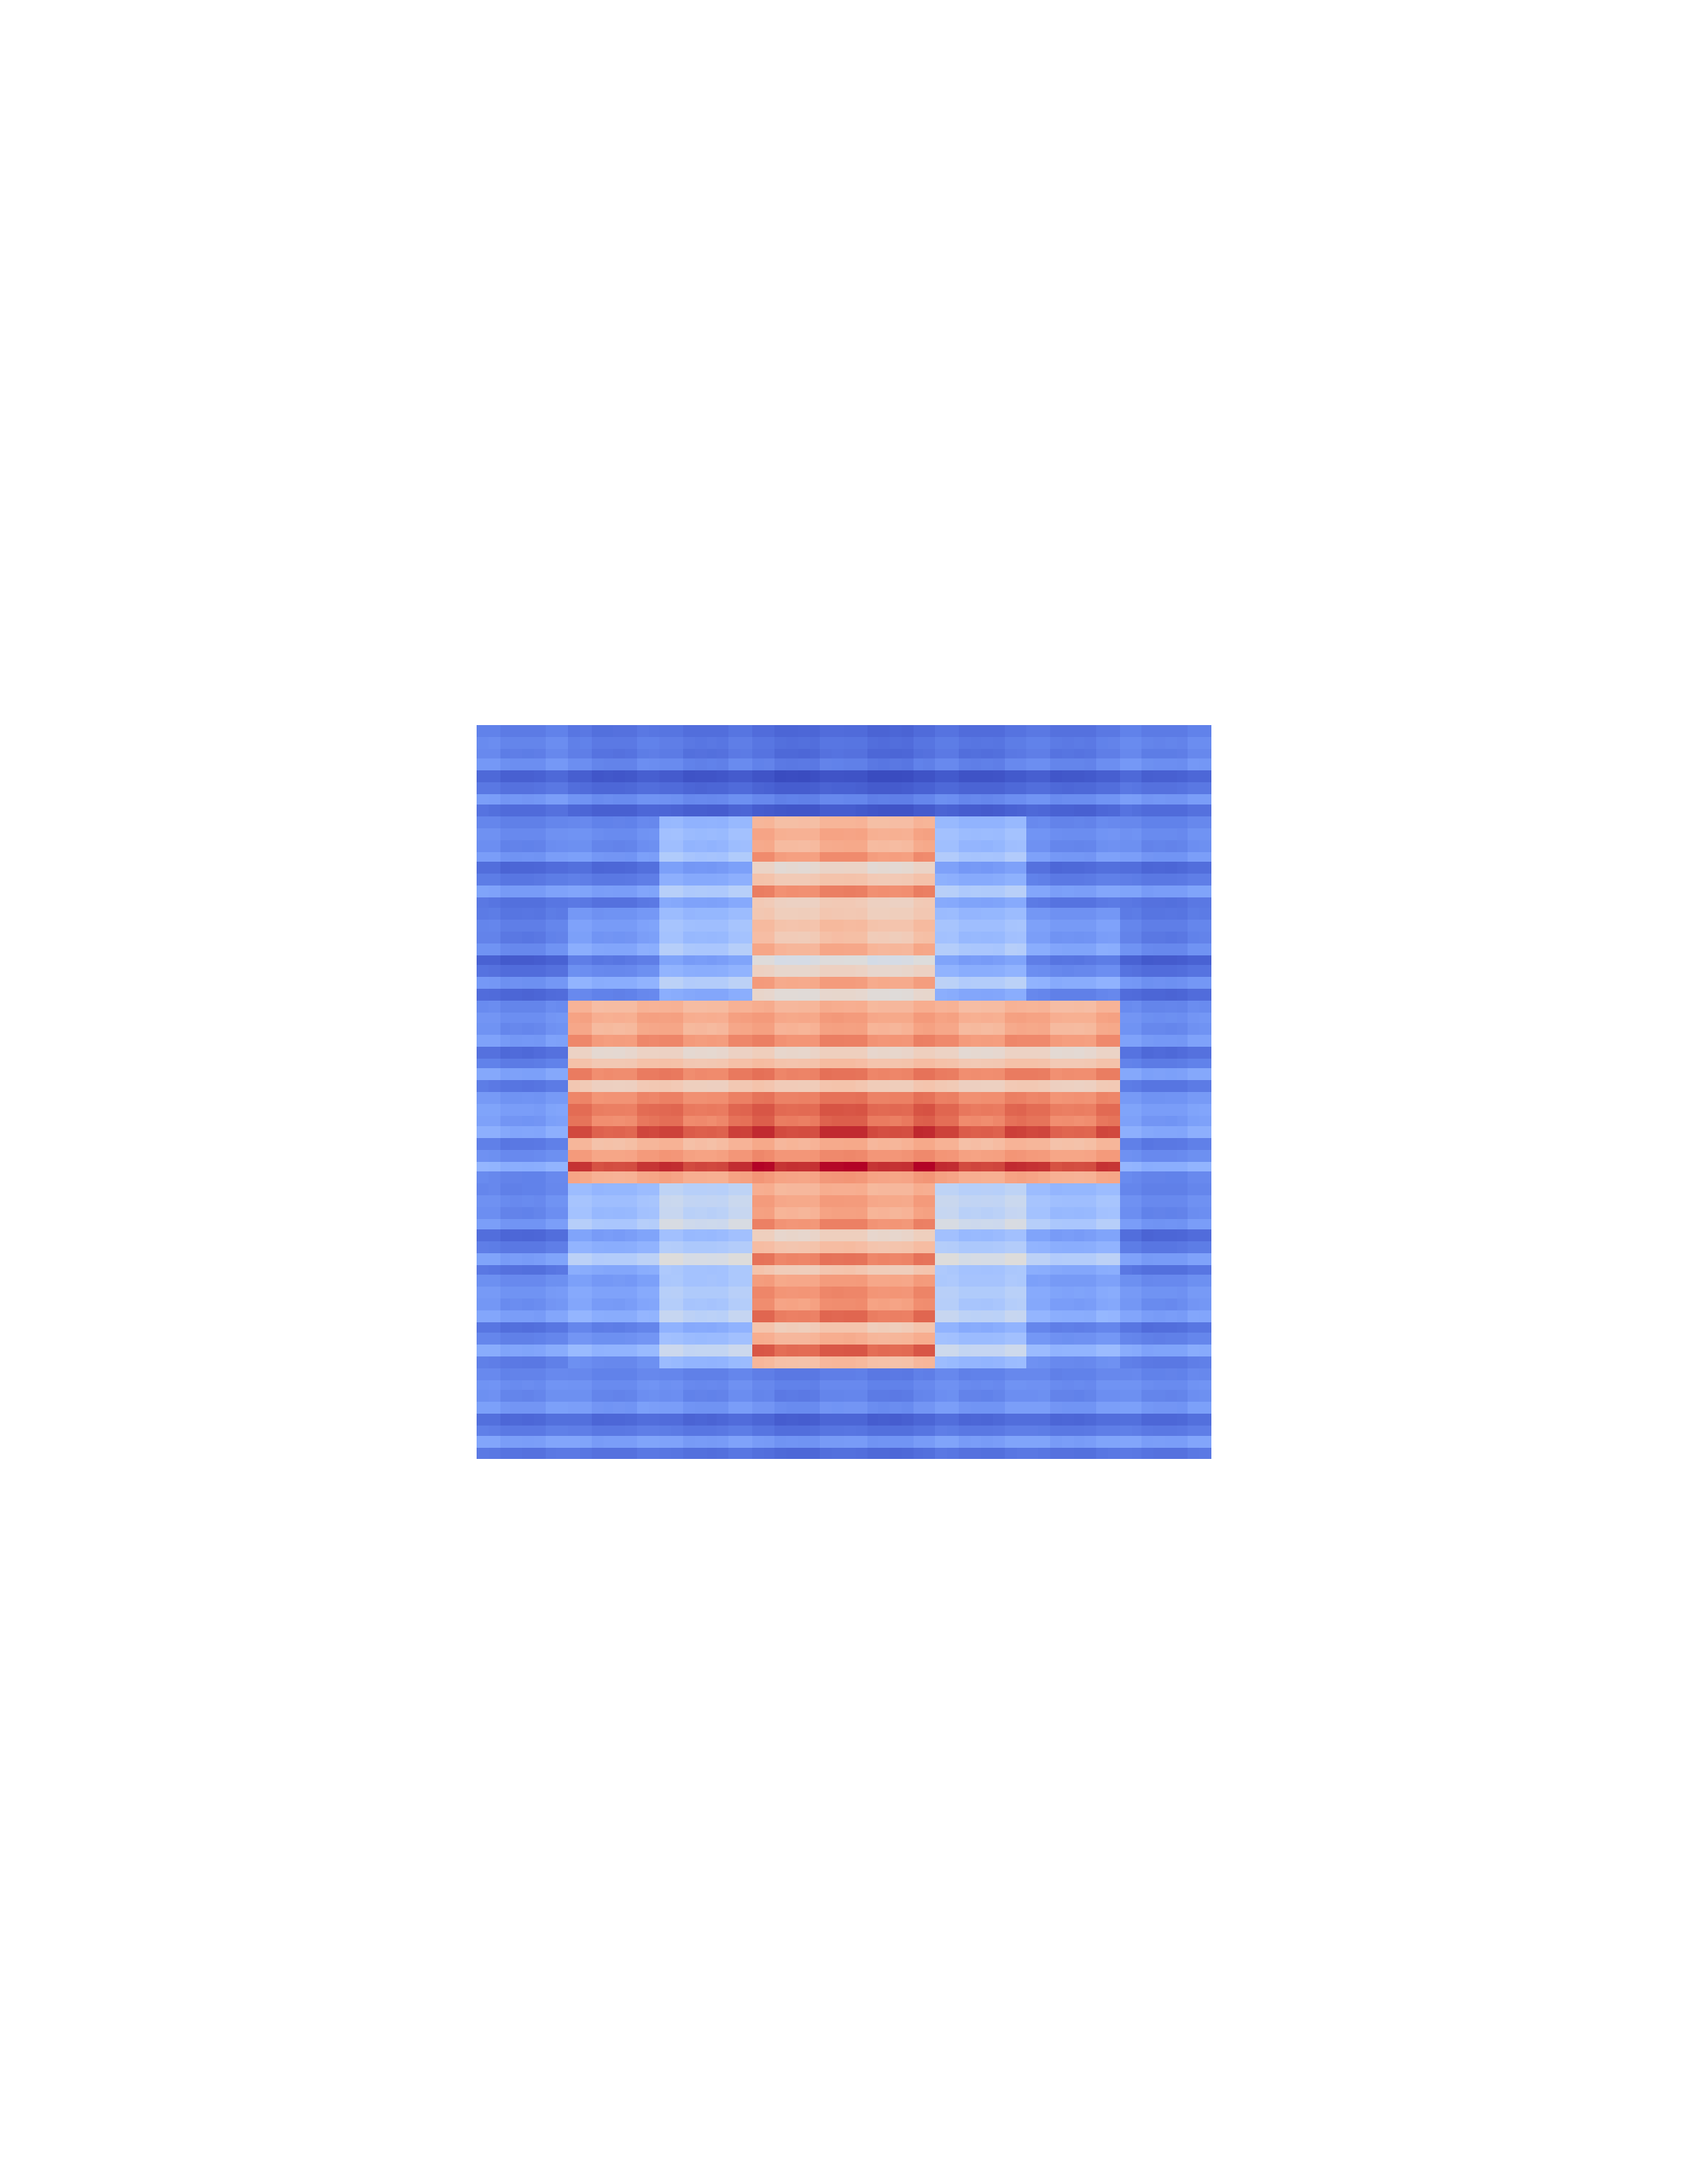}}  \quad 
        \subfigure[][d=2,R=1,N=3,P=387]{\includegraphics[height=0.3\columnwidth]{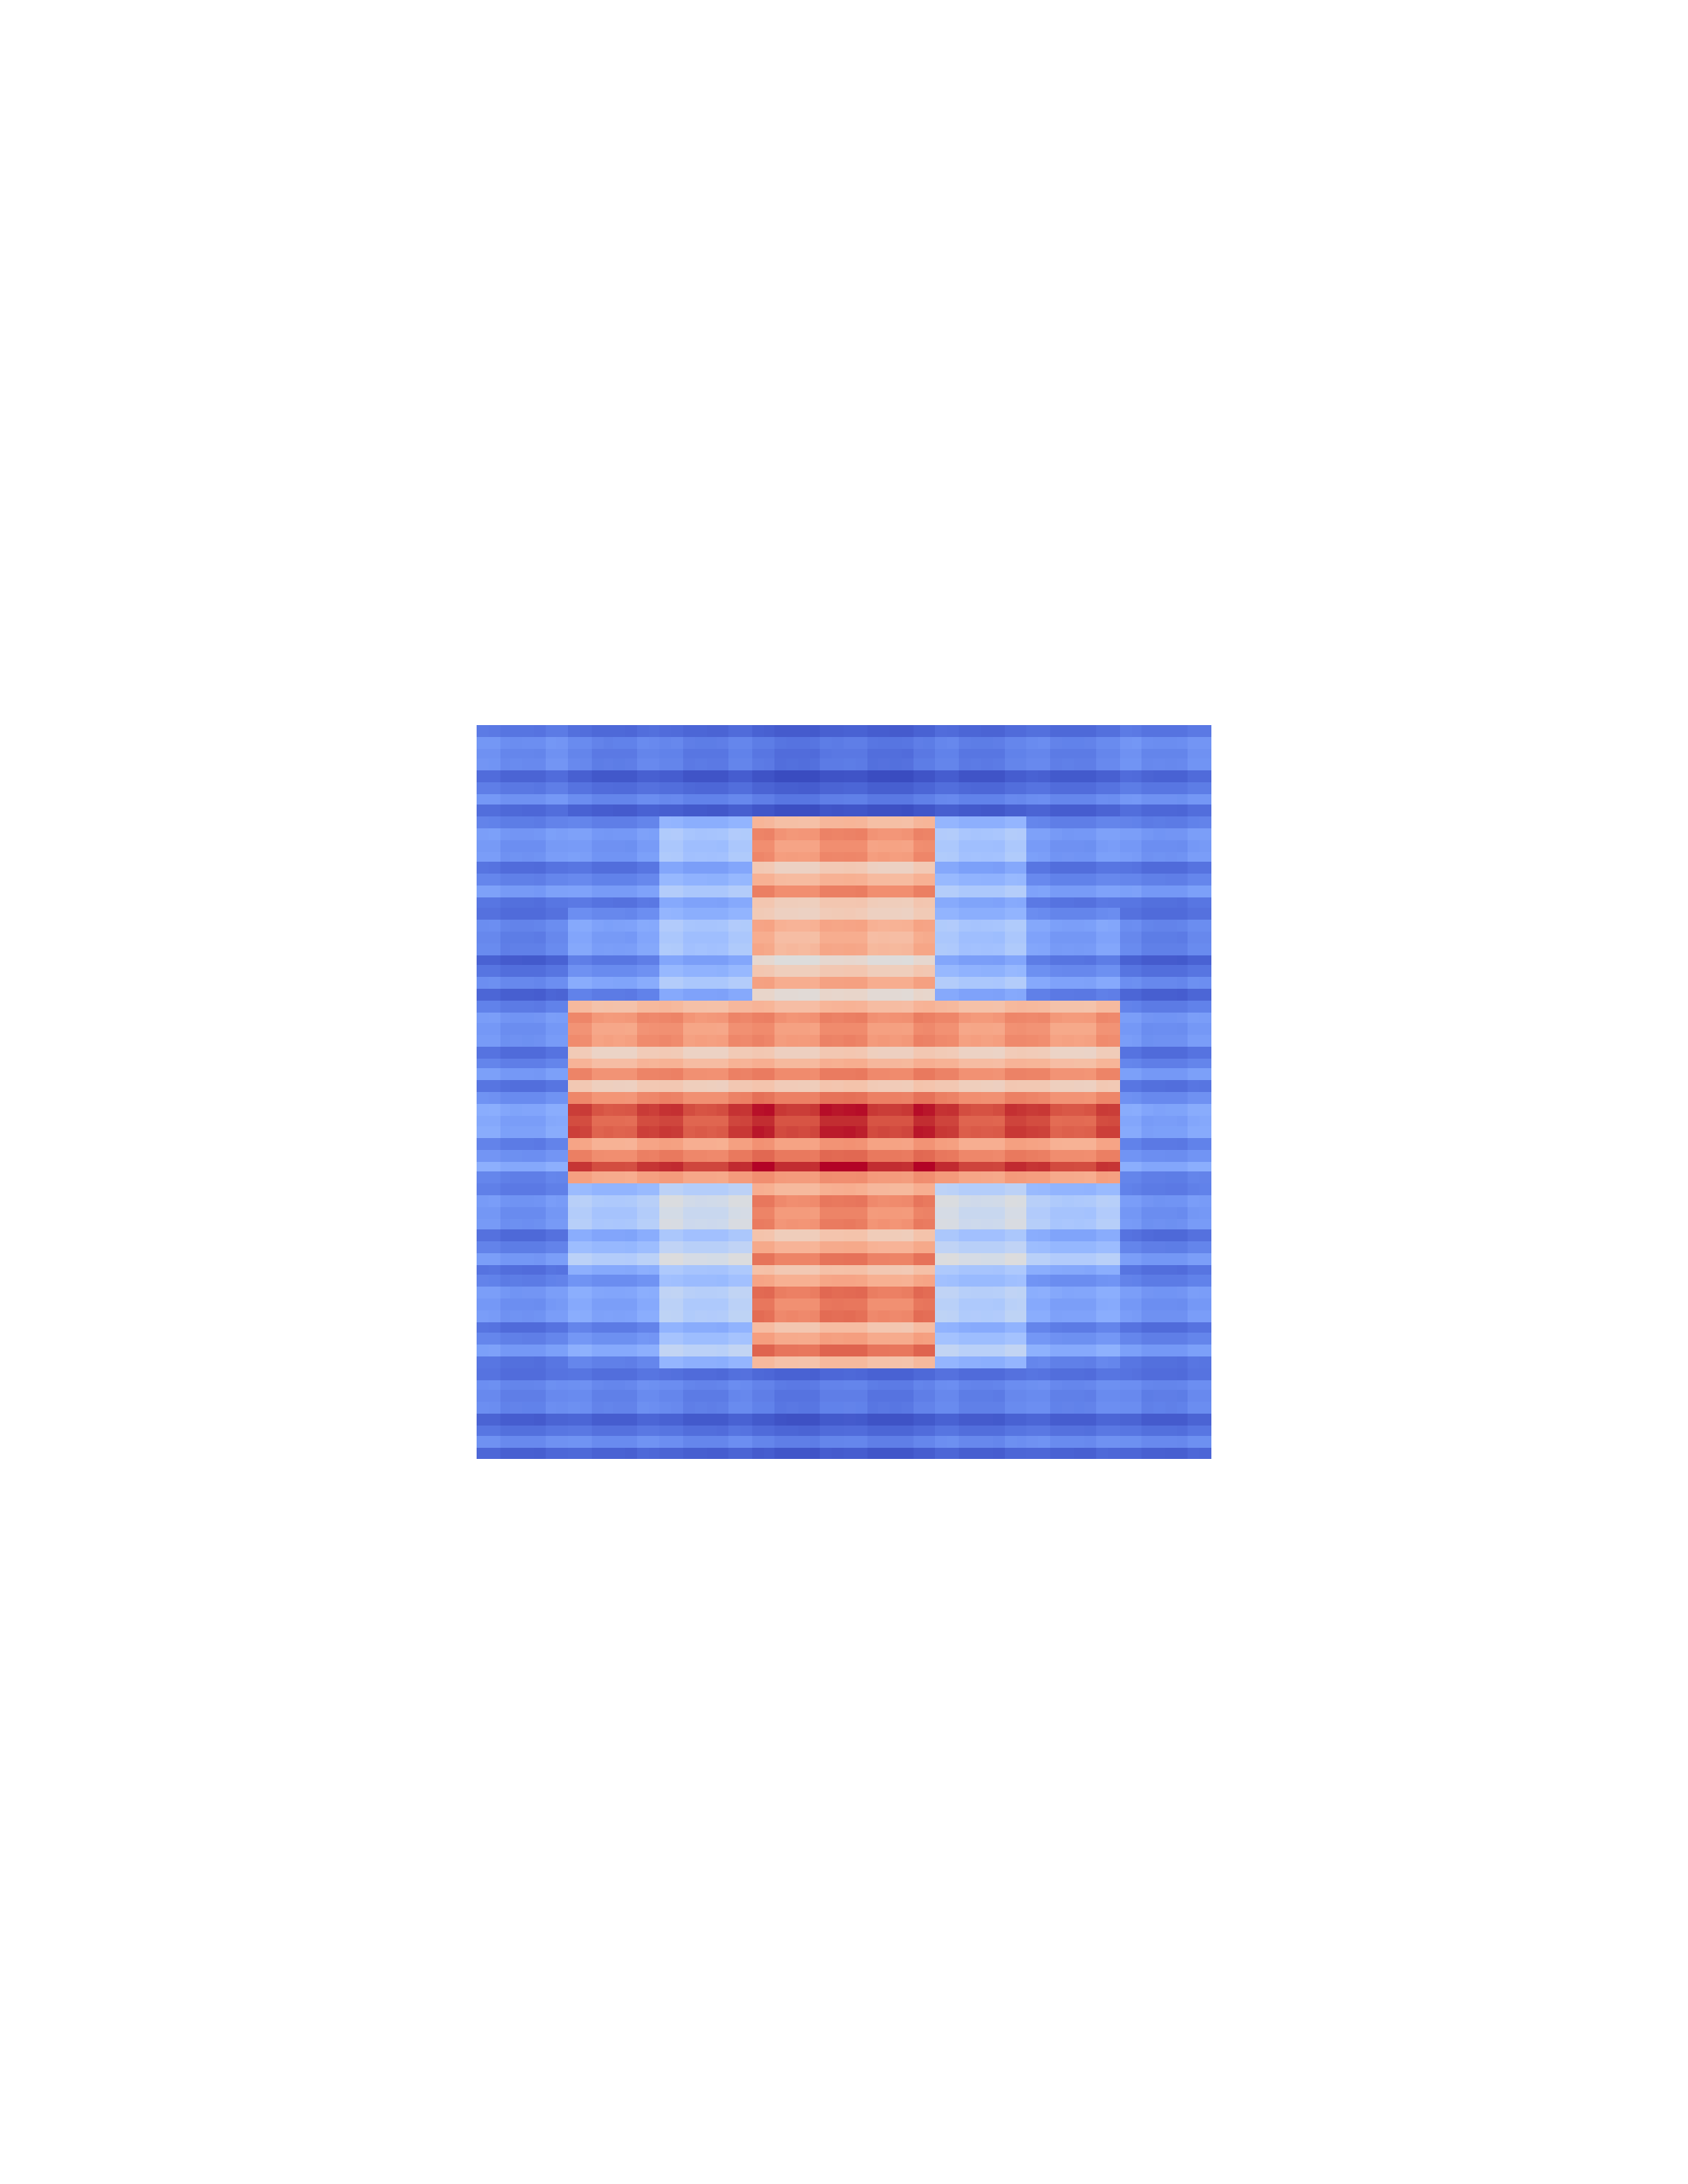}}  \quad 
        \subfigure[][d=2,R=1,N=4,P=516]{\includegraphics[height=0.3\columnwidth]{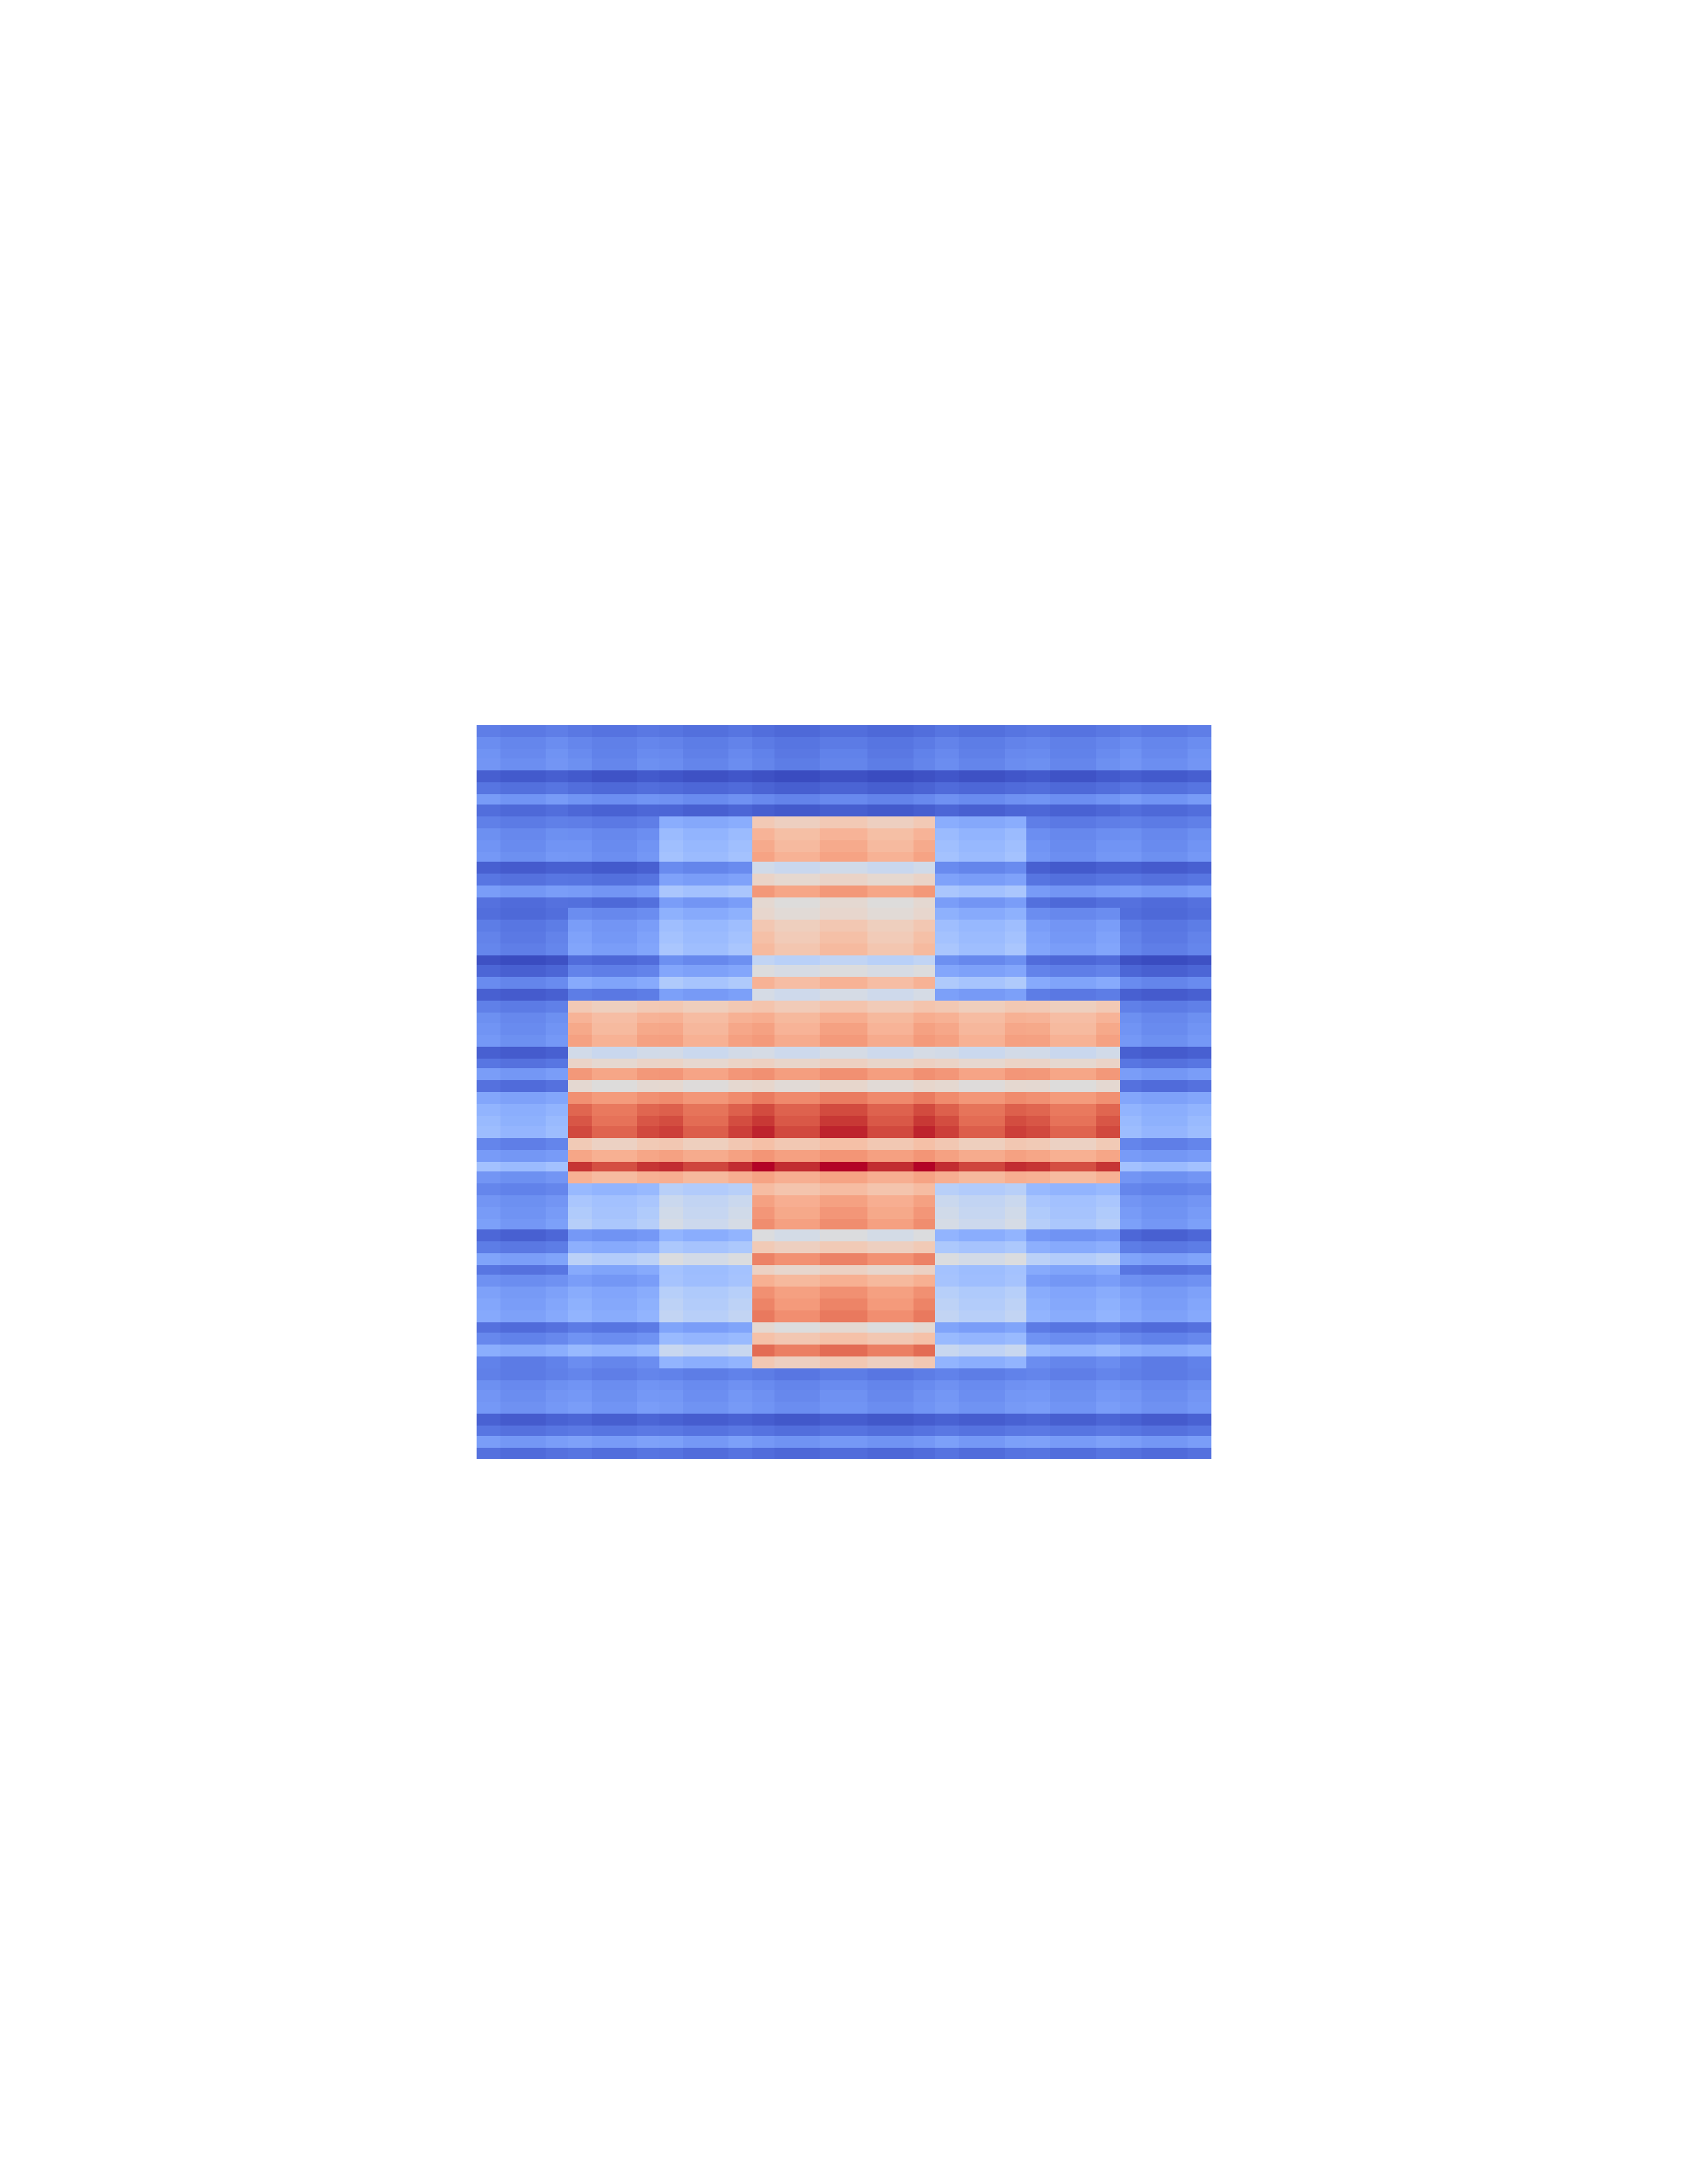}} 
        \caption{Blocks variant.}
    \end{figure*}

    \begin{figure*}
        \centering 
        \subfigure[][Original, P=4096]{\includegraphics[height=0.3\columnwidth]{pics/synthetic/original_d2_b1.eps}} \quad 
        \subfigure[][Linear Regression, P=4096]{\includegraphics[height=0.3\columnwidth]{pics/synthetic/linear_d2_b1.eps}} \quad 
        \subfigure[][d=2,R=1,N=2,P=256]{\includegraphics[height=0.3\columnwidth]{pics/synthetic/d2_R1_N2.eps}}  \quad 
        \subfigure[][d=3,R=1,N=2,P=98]{\includegraphics[height=0.3\columnwidth]{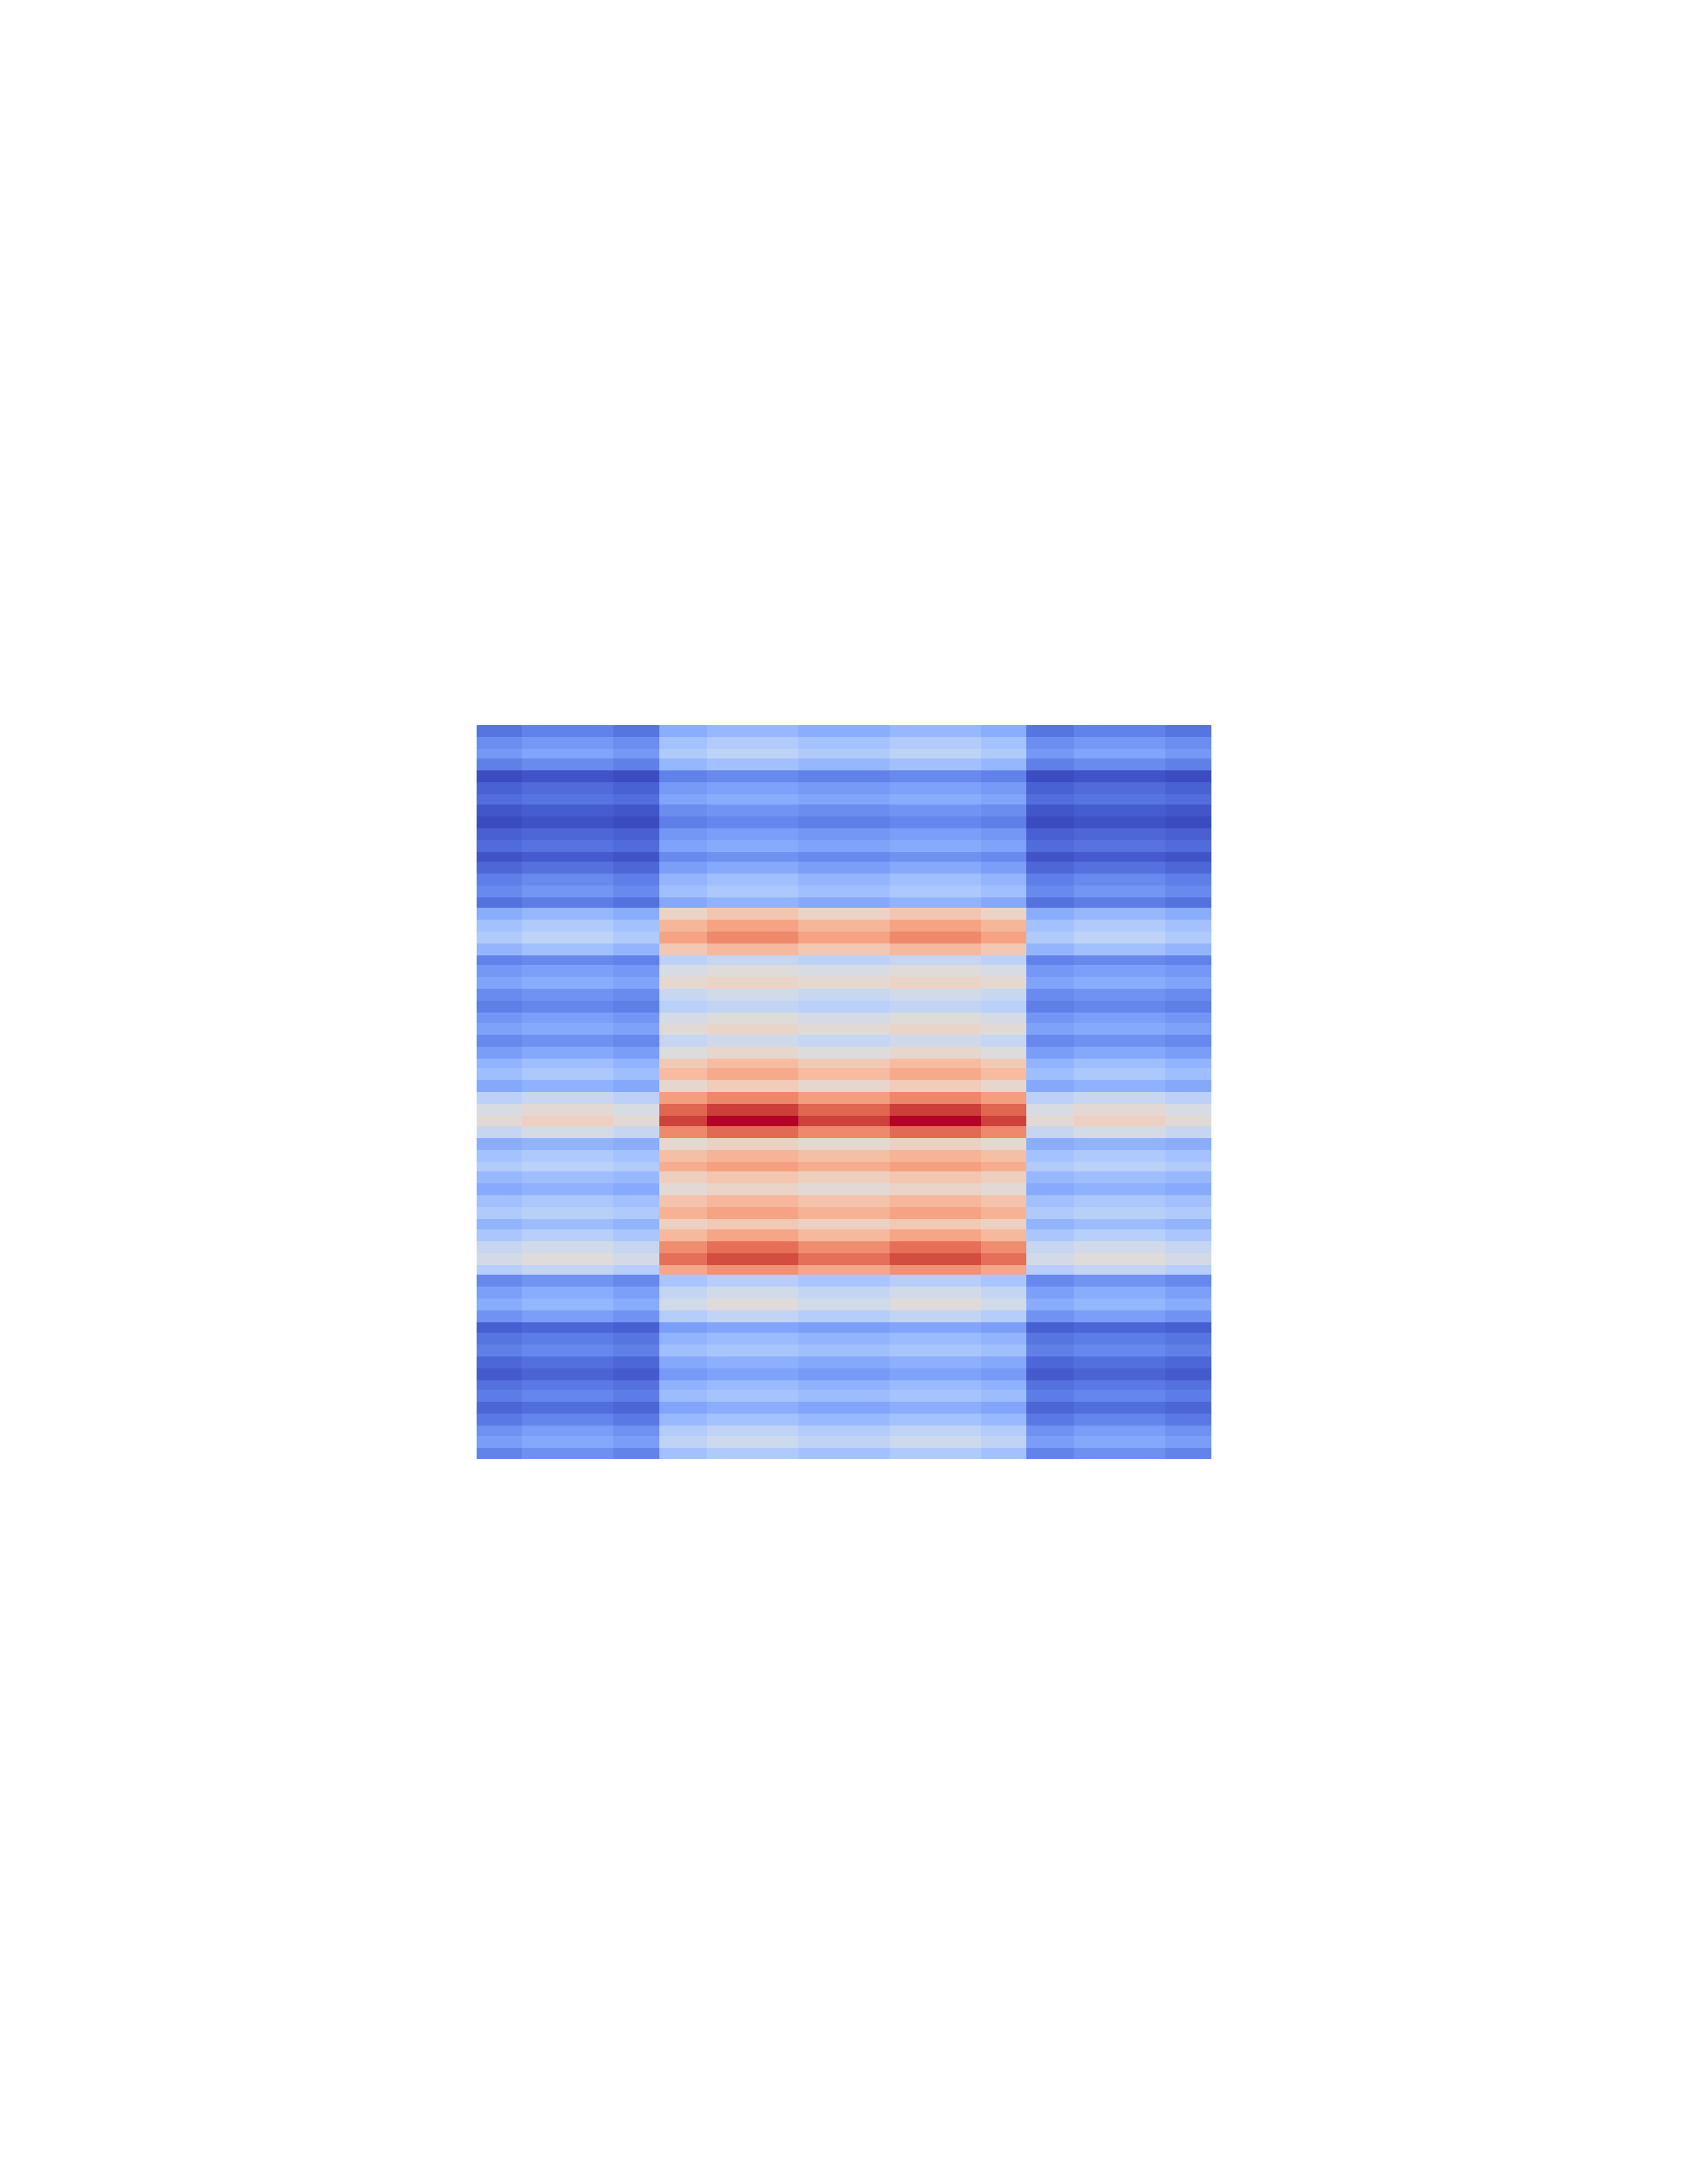}}  \quad 
        \subfigure[][d=4,R=1,N=2,P=66]{\includegraphics[height=0.3\columnwidth]{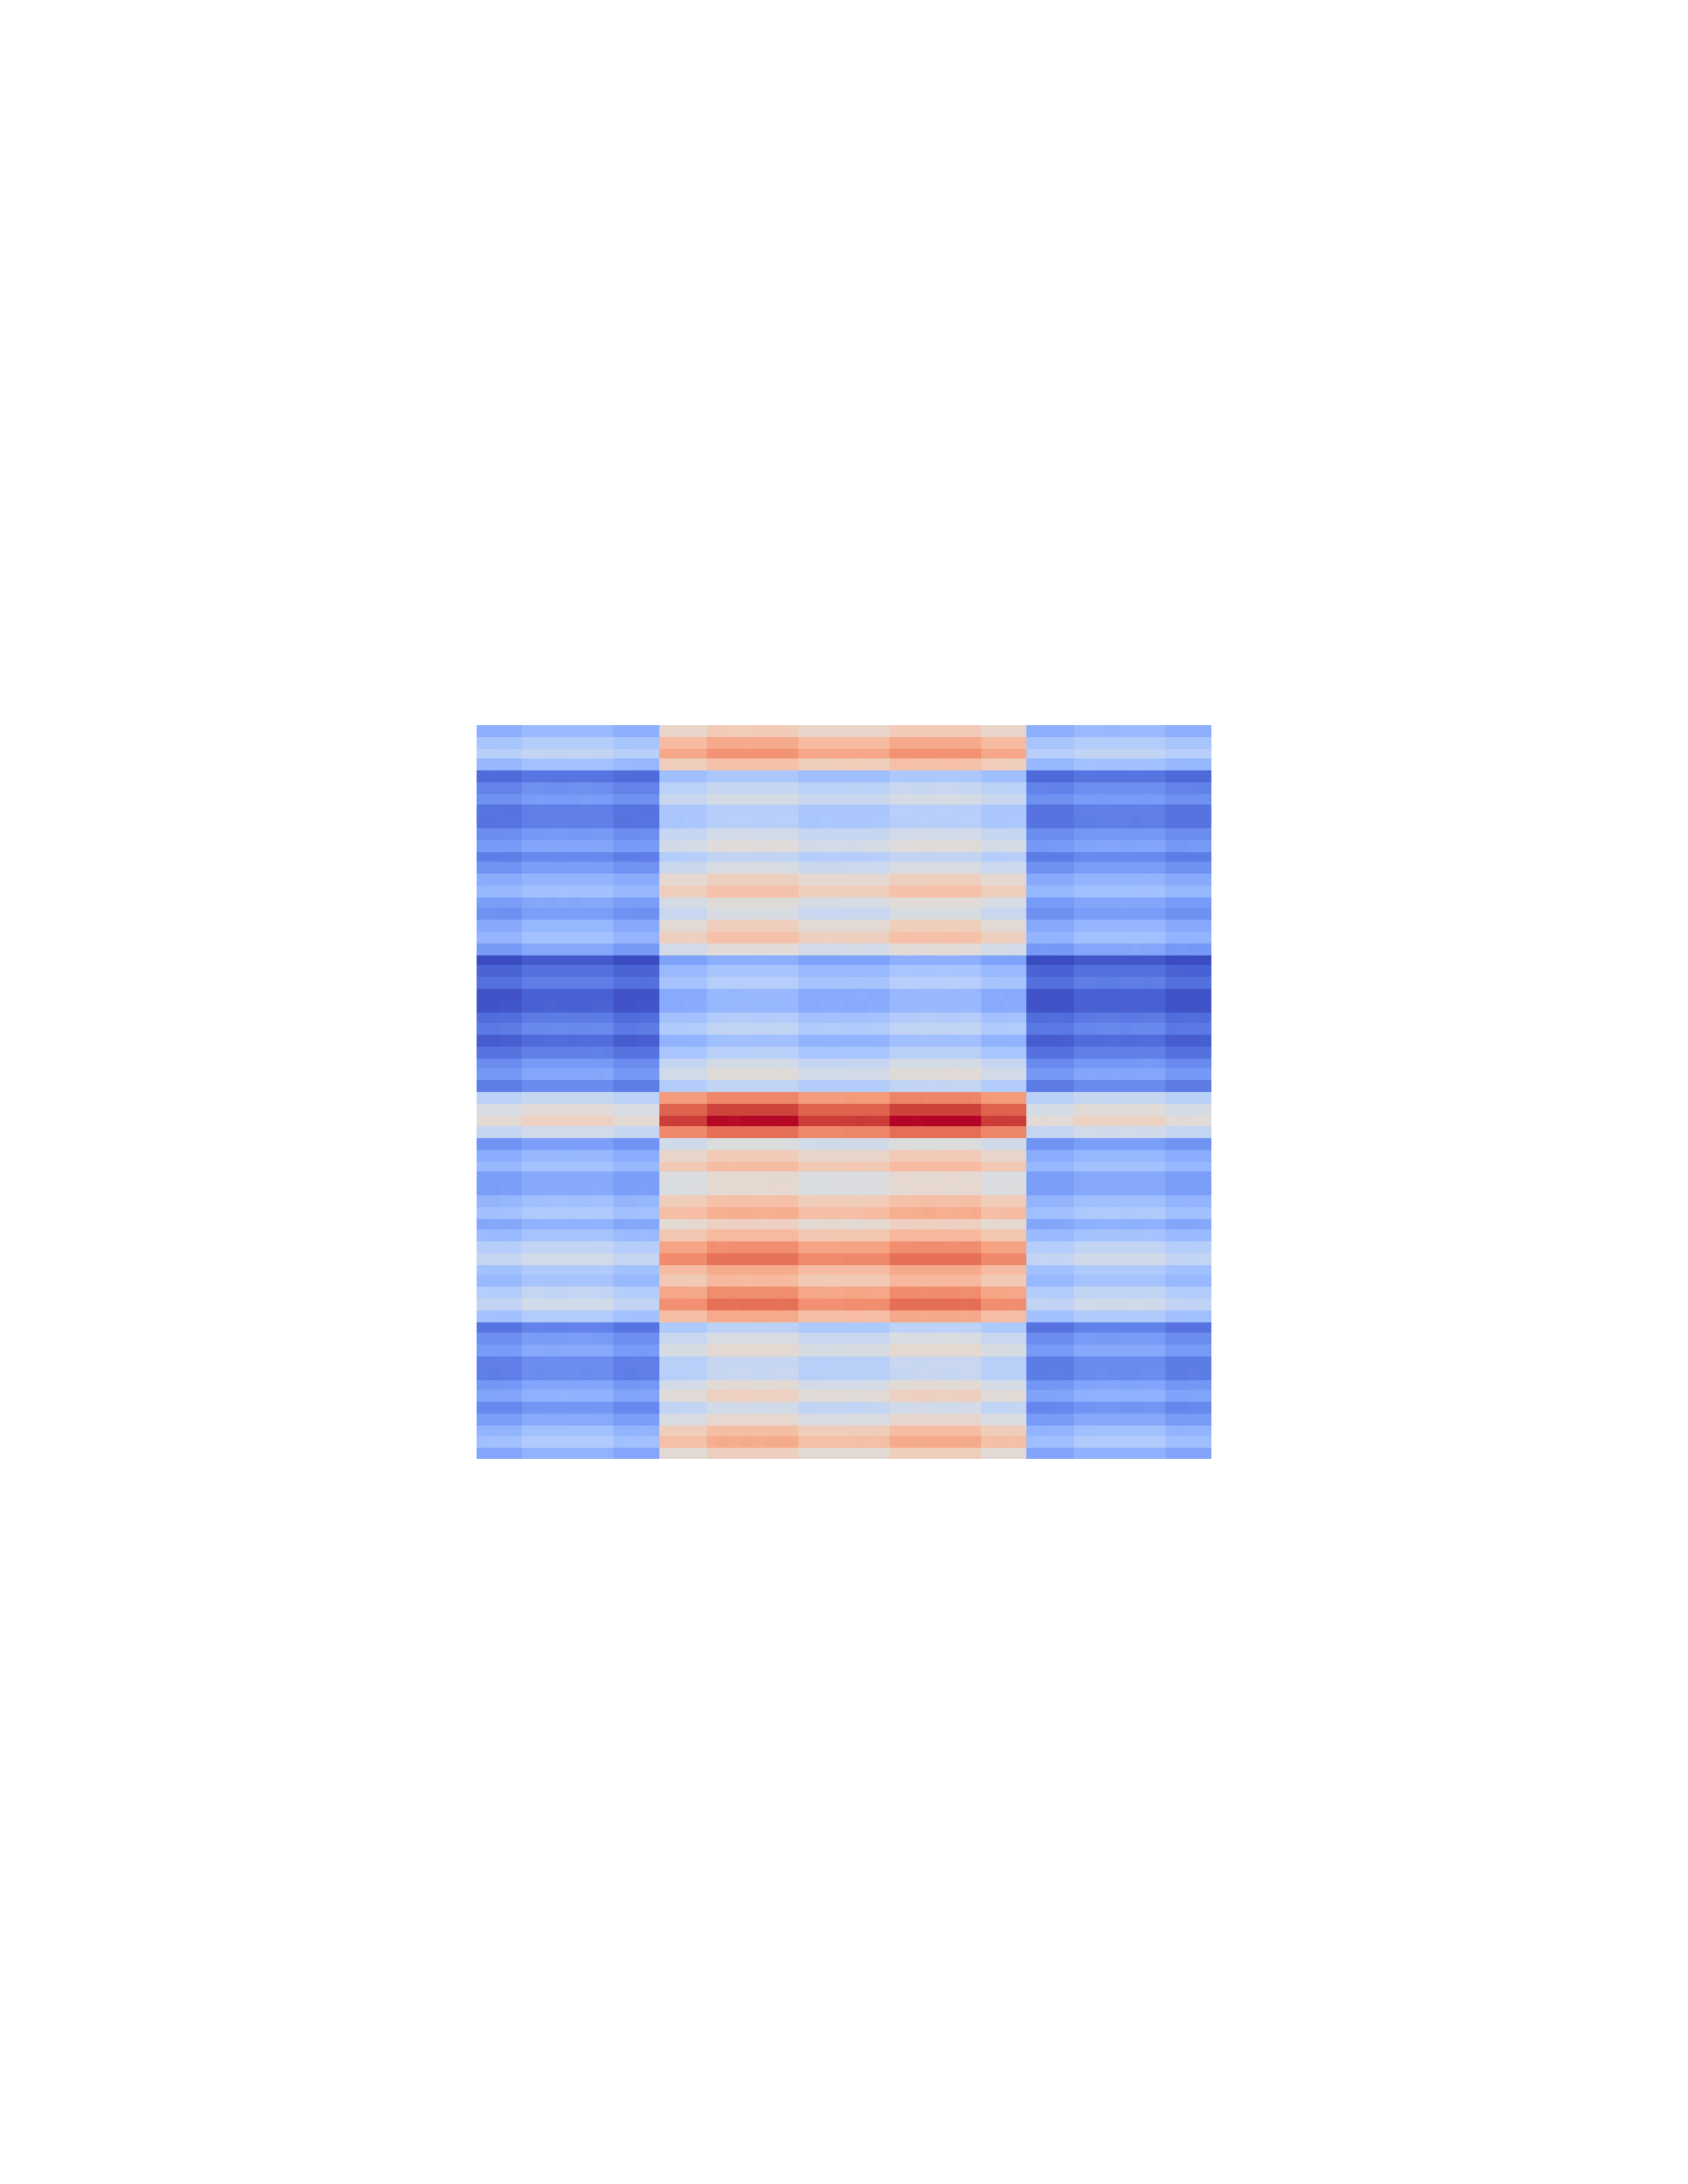}}  \quad 
        \subfigure[][d=5,R=1,N=2,P=42]{\includegraphics[height=0.3\columnwidth]{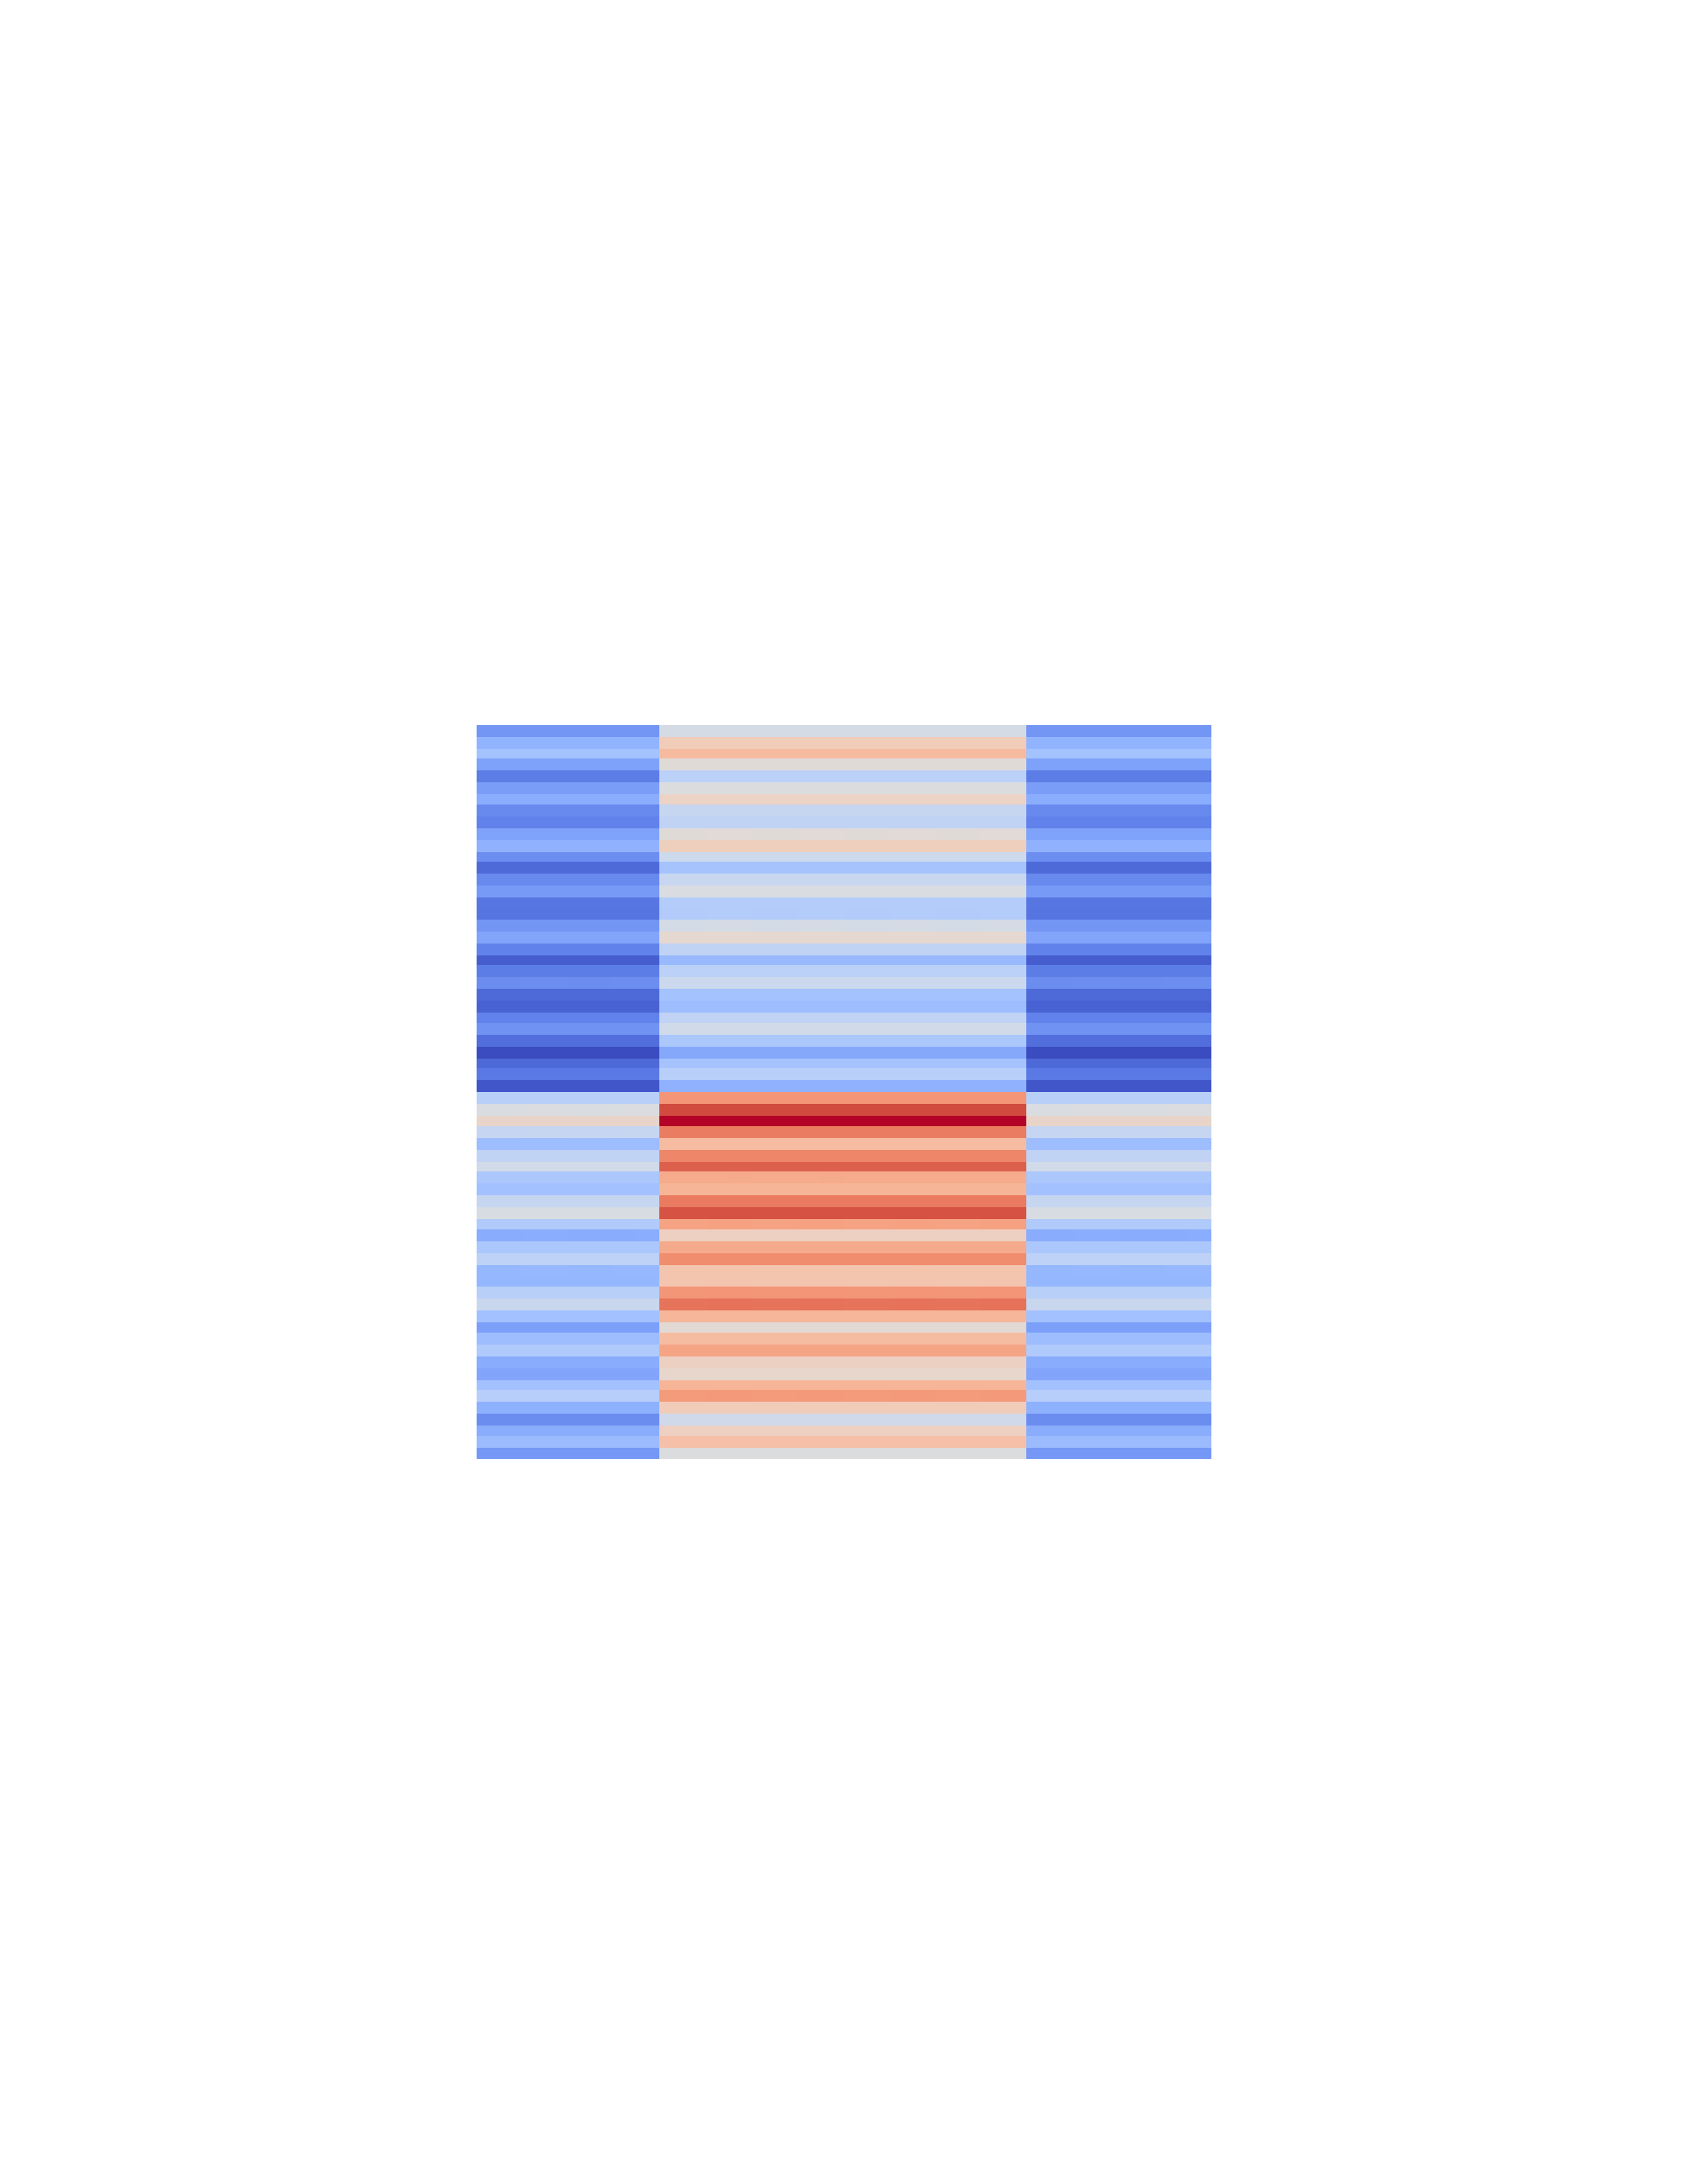}} 
        \caption{$d$ variant.}
    \end{figure*}

    \newpage
    \null
    \newpage

    \begin{figure*}
        \centering
        \subfigure[][Original, P=4096]{\includegraphics[height=0.3\columnwidth]{pics/synthetic/original_d2_b1.eps}} \quad 
        \subfigure[][Linear Regression, P=4096]{\includegraphics[height=0.3\columnwidth]{pics/synthetic/linear_d2_b1.eps}} \quad 
        \subfigure[][d=2, R=1, P=128]{\includegraphics[height=0.3\columnwidth]{pics/imgs_tt1/d2_R1.eps}}  \quad
        \subfigure[][d=2, R=2, P=256]{\includegraphics[height=0.3\columnwidth]{pics/imgs_tt1/d2_R2.eps}}  \quad
        \subfigure[][d=2, R=3, P=384]{\includegraphics[height=0.3\columnwidth]{pics/imgs_tt1/d2_R3.eps}}  \quad
        \subfigure[][d=2, R=4, P=512]{\includegraphics[height=0.3\columnwidth]{pics/imgs_tt1/d2_R4.eps}} \\

        \subfigure[][Original, P=4096]{\includegraphics[height=0.3\columnwidth]{pics/synthetic/original_d2_b1.eps}} \quad 
        \subfigure[][Linear Regression, P=4096]{\includegraphics[height=0.3\columnwidth]{pics/synthetic/linear_d2_b1.eps}} \quad 
        \subfigure[][d=3, R=1, P=48]{\includegraphics[height=0.3\columnwidth]{pics/imgs_tt1/d3_R1.eps}}  \quad
        \subfigure[][d=3, R=2, P=128]{\includegraphics[height=0.3\columnwidth]{pics/imgs_tt1/d3_R2.eps}}  \quad
        \subfigure[][d=3, R=3, P=240]{\includegraphics[height=0.3\columnwidth]{pics/imgs_tt1/d3_R3.eps}}  \quad
        \subfigure[][d=3, R=4, P=384]{\includegraphics[height=0.3\columnwidth]{pics/imgs_tt1/d3_R4.eps}} \\

        \subfigure[][Original]{\includegraphics[height=0.3\columnwidth]{pics/synthetic/original_d2_b1.eps}} \quad 
        \subfigure[][Linear Regression]{\includegraphics[height=0.3\columnwidth]{pics/synthetic/linear_d2_b1.eps}} \quad 
        \subfigure[][d=4, R=1, P=32]{\includegraphics[height=0.3\columnwidth]{pics/imgs_tt1/d4_R1.eps}}  \quad
        \subfigure[][d=4, R=2, P=96]{\includegraphics[height=0.3\columnwidth]{pics/imgs_tt1/d4_R2.eps}}  \quad
        \subfigure[][d=4, R=3, P=192]{\includegraphics[height=0.3\columnwidth]{pics/imgs_tt1/d4_R3.eps}}  \quad
        \subfigure[][d=4, R=4, P=320]{\includegraphics[height=0.3\columnwidth]{pics/imgs_tt1/d4_R4.eps}} \\

        \subfigure[][Original, P=4096]{\includegraphics[height=0.3\columnwidth]{pics/synthetic/original_d2_b1.eps}} \quad 
        \subfigure[][Linear Regression, P=4096]{\includegraphics[height=0.3\columnwidth]{pics/synthetic/linear_d2_b1.eps}} \quad 
        \subfigure[][d=5, R=1, P=20]{\includegraphics[height=0.3\columnwidth]{pics/imgs_tt1/d5_R1.eps}}  \quad
        \subfigure[][d=5, R=2, P=64]{\includegraphics[height=0.3\columnwidth]{pics/imgs_tt1/d5_R2.eps}}  \quad
        \subfigure[][d=5, R=3, P=132]{\includegraphics[height=0.3\columnwidth]{pics/imgs_tt1/d5_R3.eps}}  \quad
        \subfigure[][d=5, R=4, P=224]{\includegraphics[height=0.3\columnwidth]{pics/imgs_tt1/d5_R4.eps}}
        \caption{Result of Tensor-Train method. Parameters $P = (\sqrt[d]{64})^2 * R^2$}
    \end{figure*}
