# Supplementary material for: Learning Compact Recurrent Neural Networks with Block-Term Tensor Decomposition
Source: arXiv:1712.05134 source file (2018-05-11)
Supplement: Supplementary file 2 [file supplement1.tex]

\clearpage
\onecolumn
\section*{Supplements}

\subsection*{1. Additional results of UCF11}

\begin{figure*}[h]
        \centering
        \subfigure[][Training Loss]{\includegraphics[height=0.14\columnwidth]{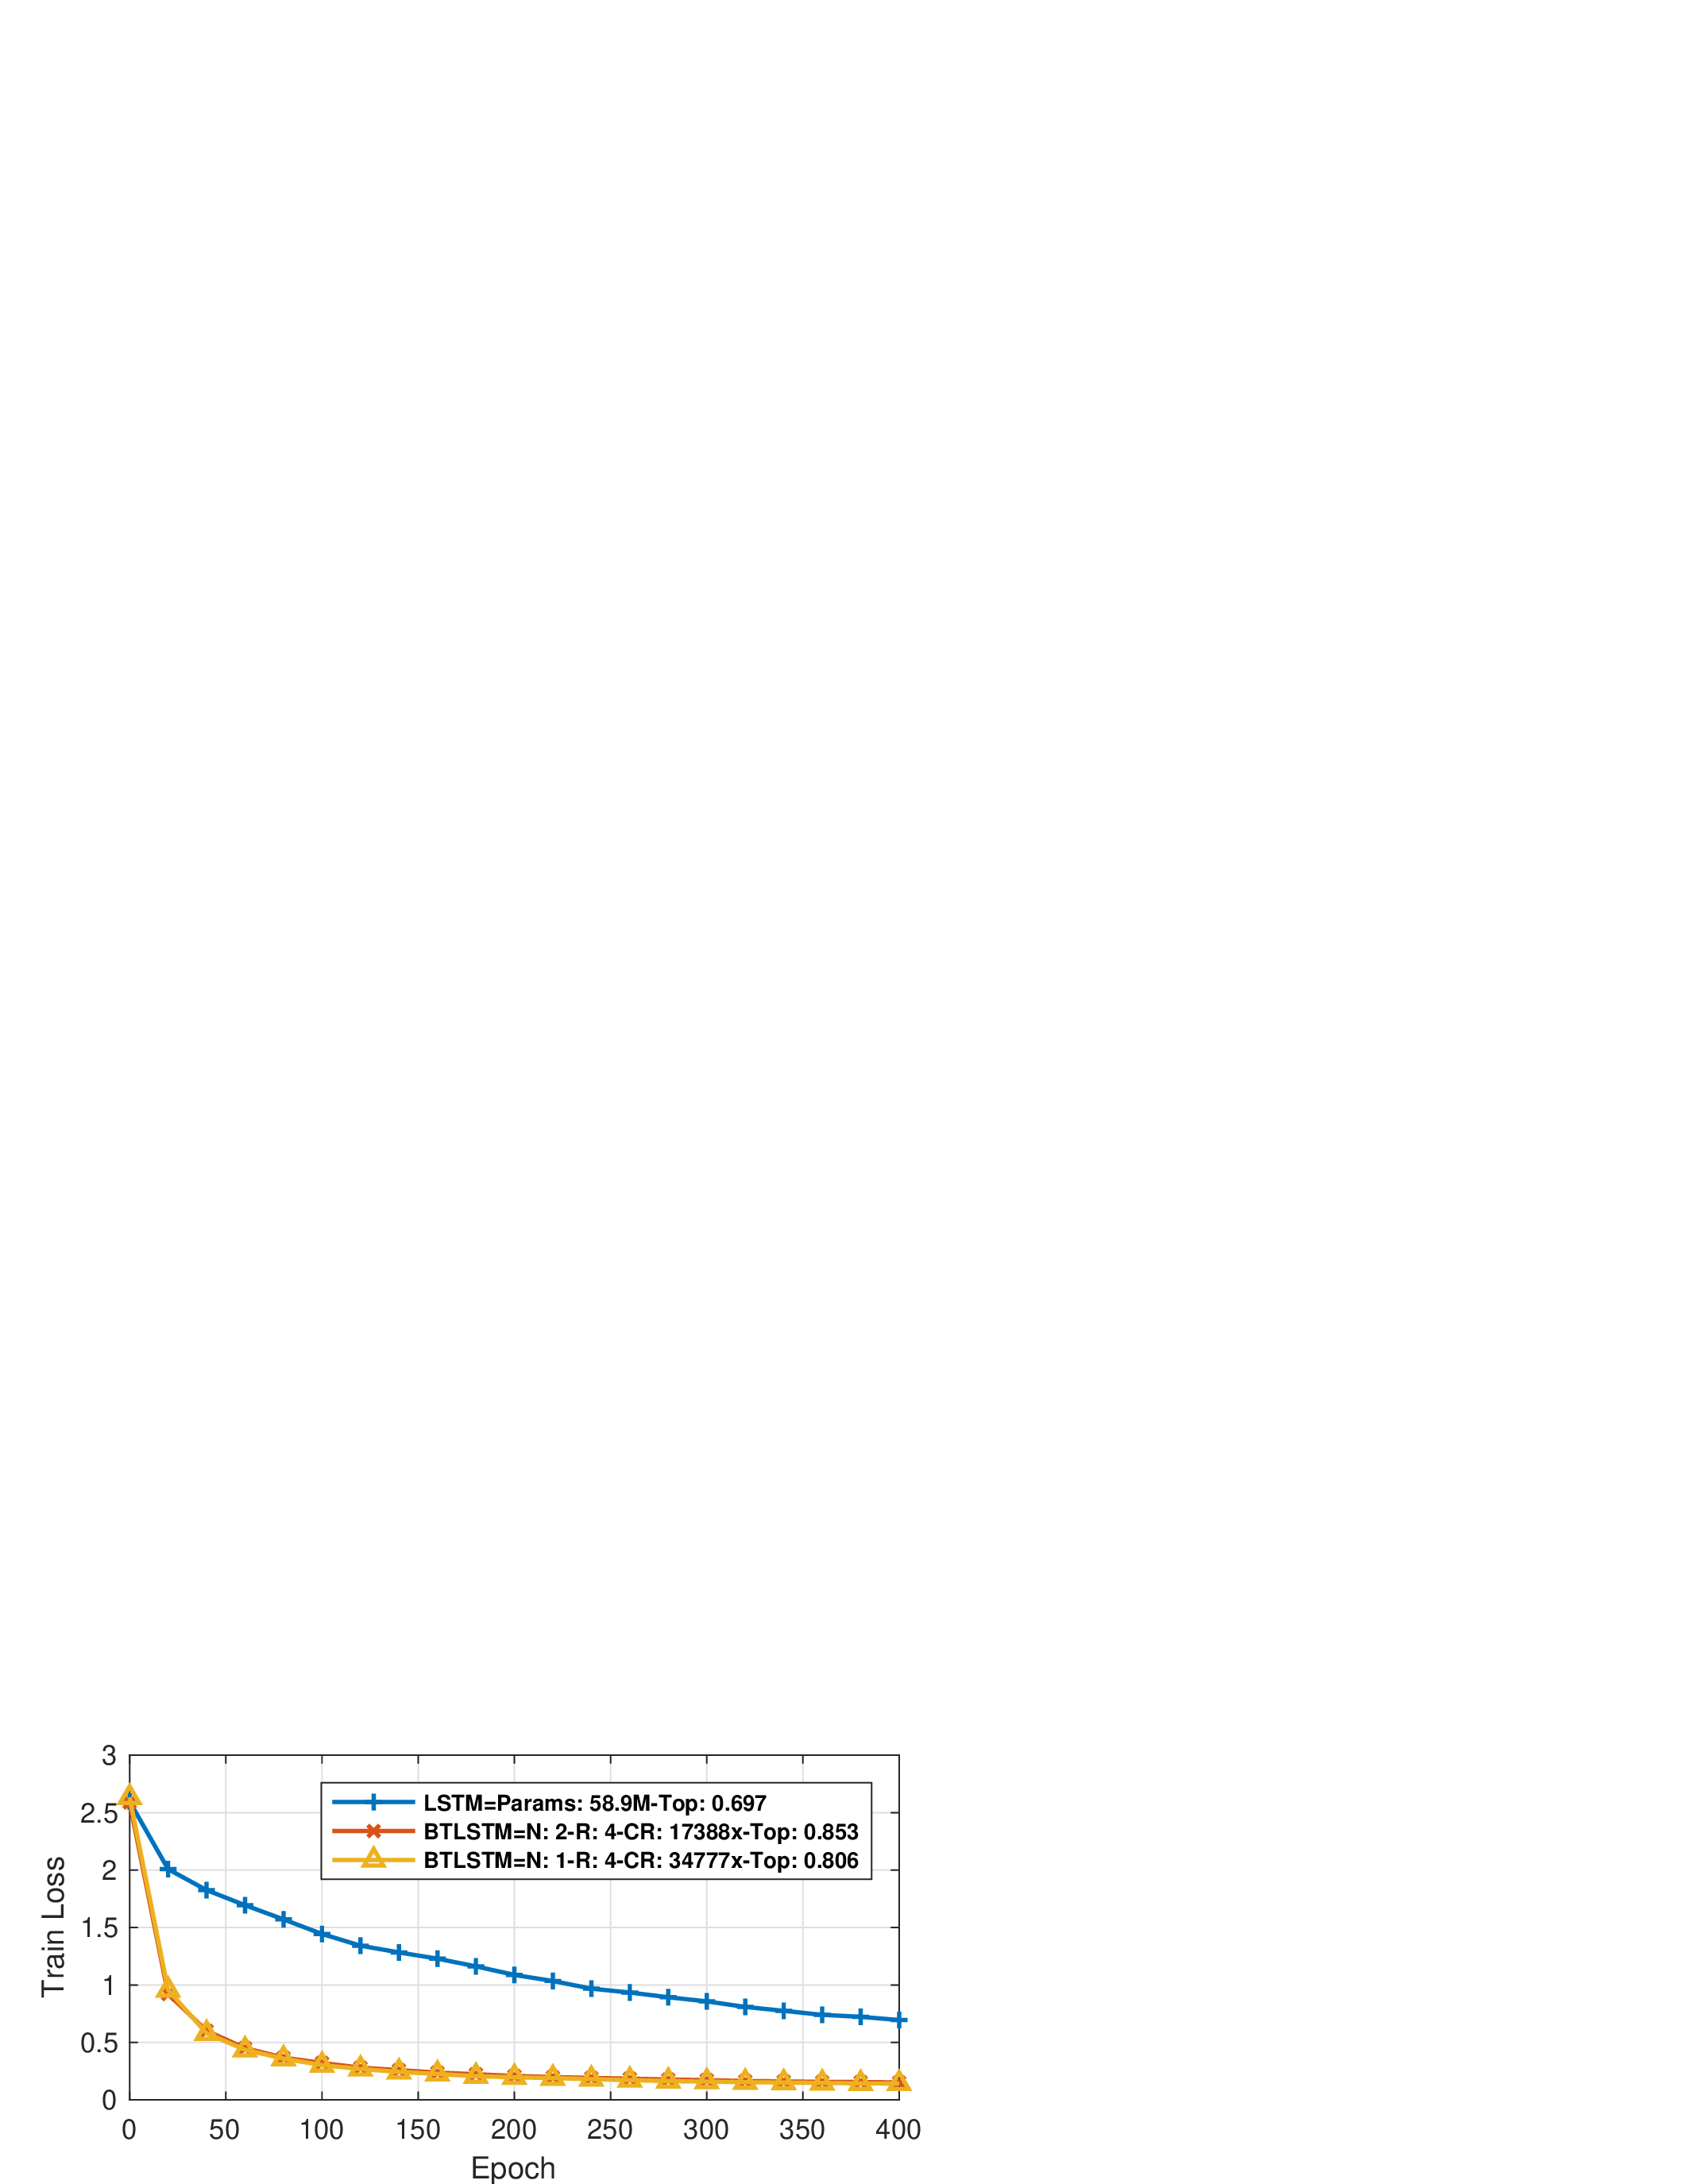}} \quad
        \subfigure[][Training Accuracy]{\includegraphics[height=0.14\columnwidth]{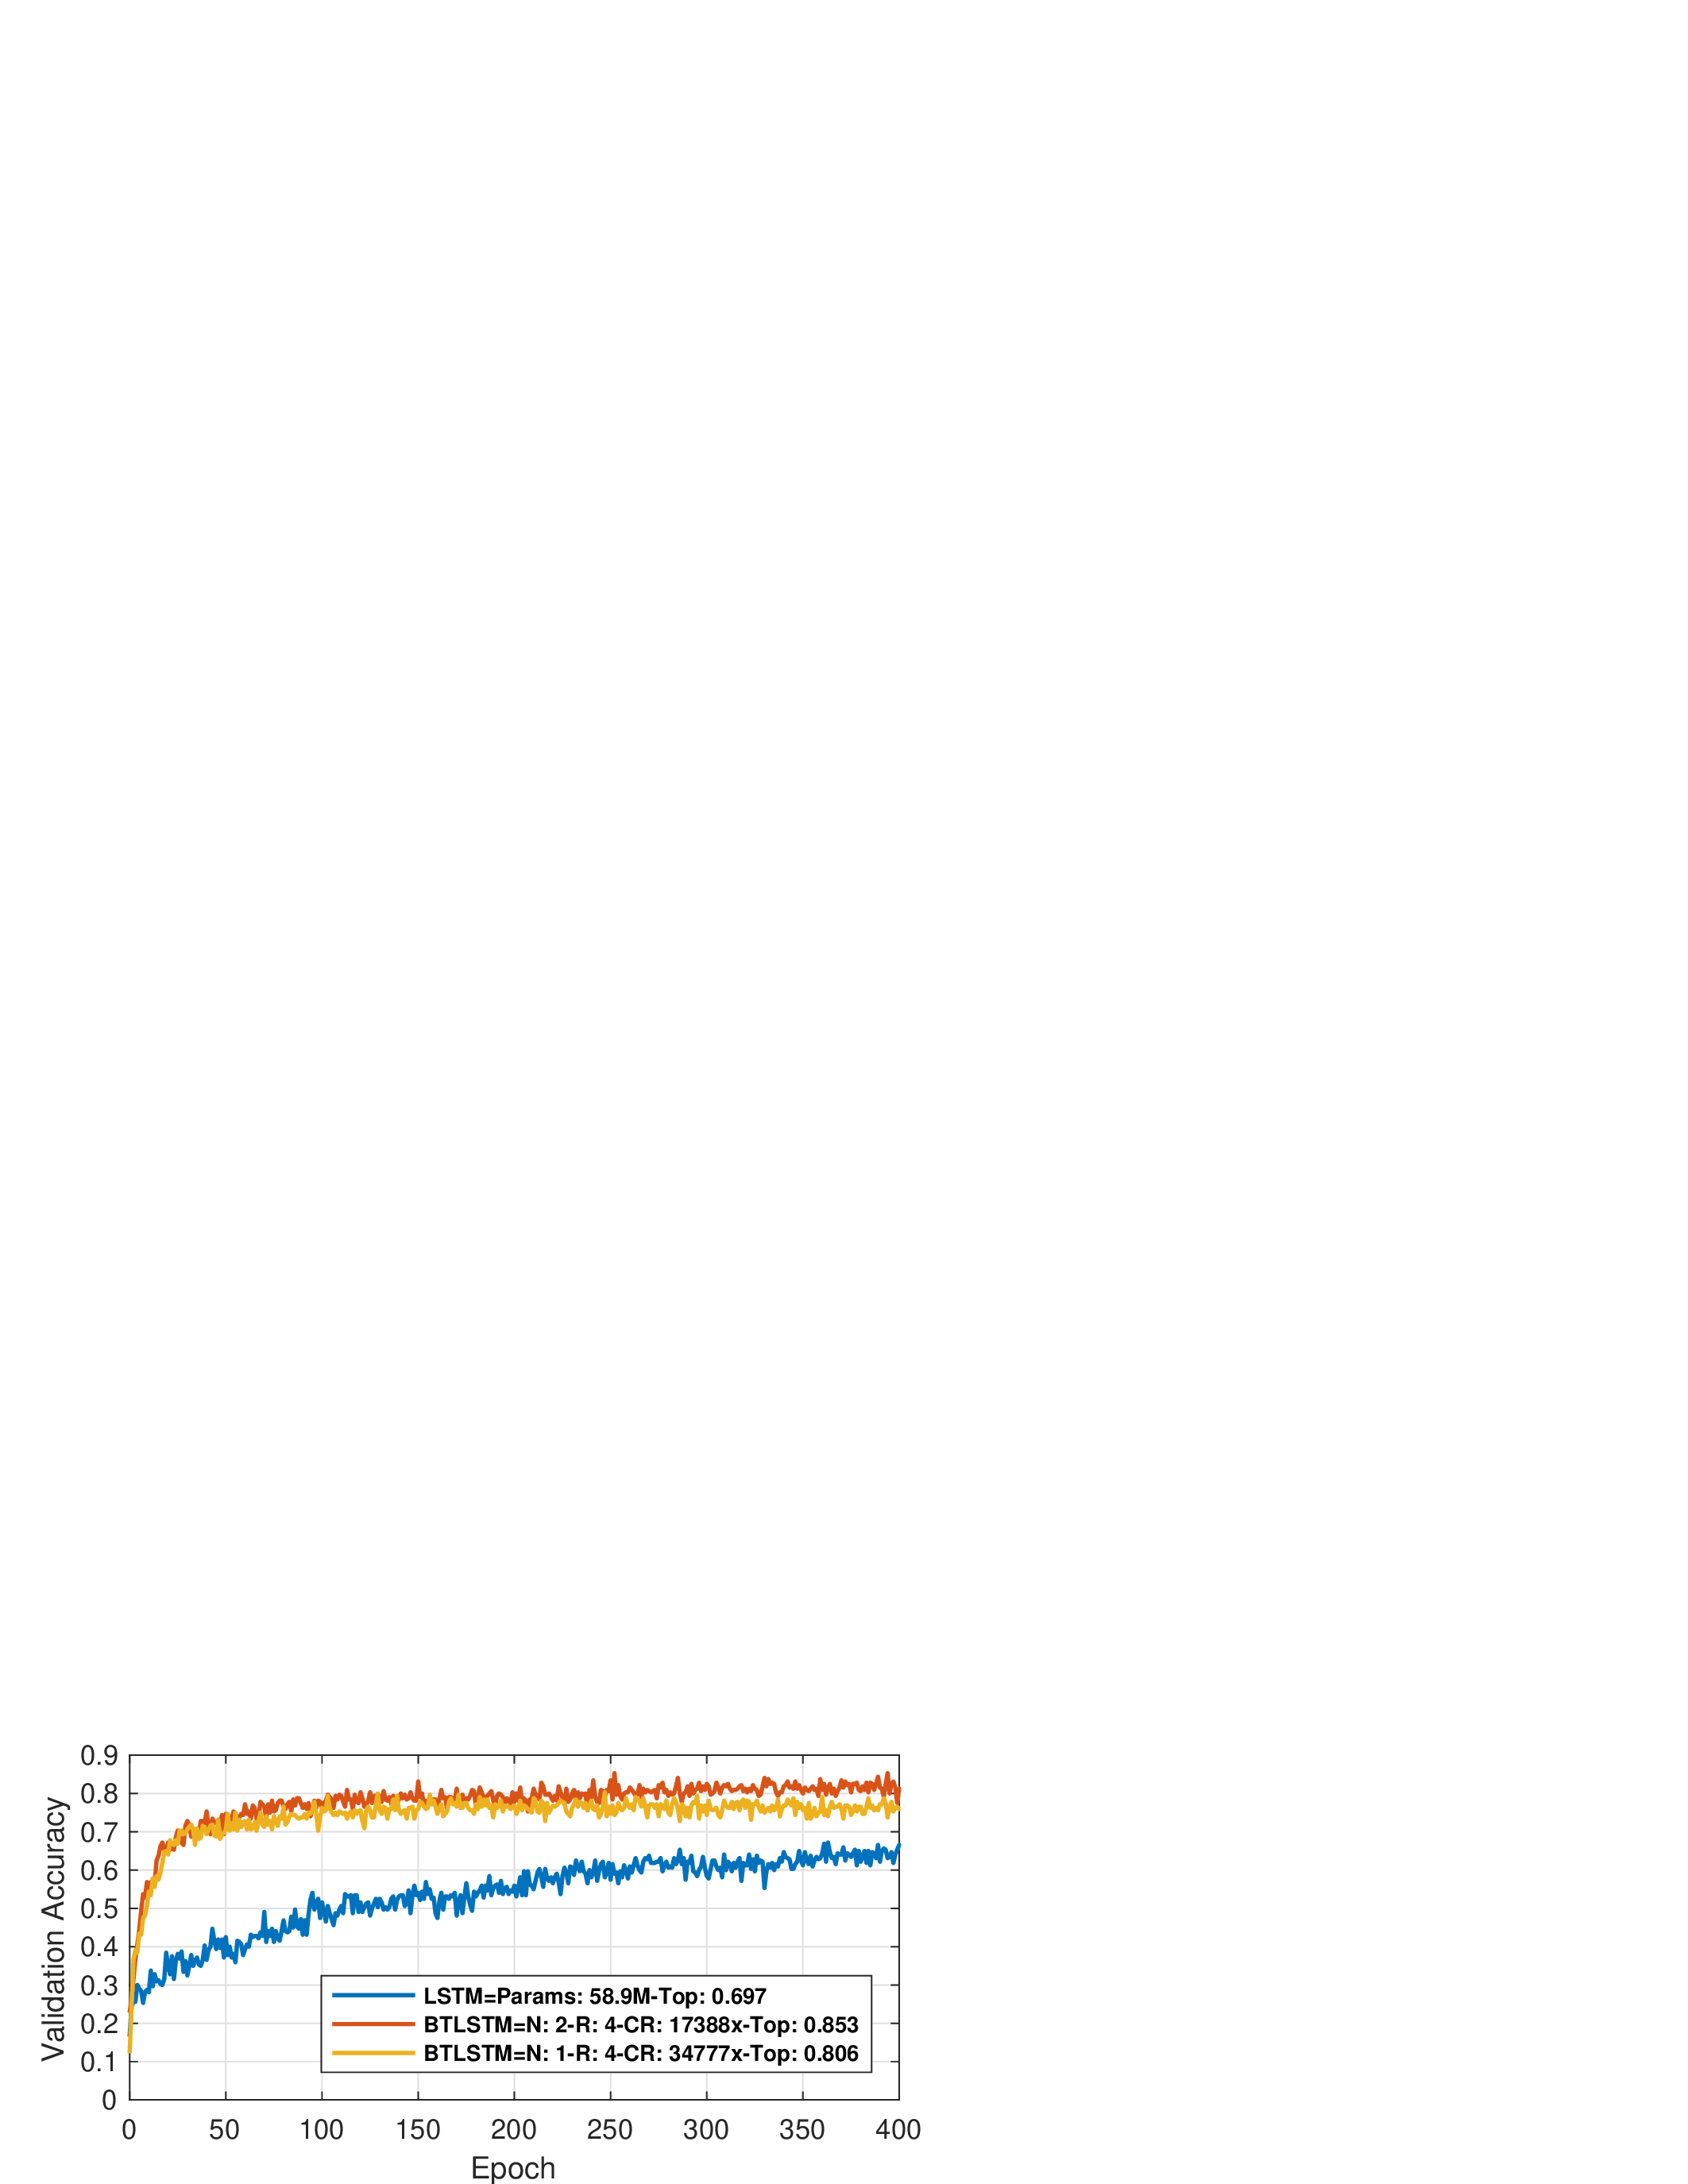}}
        \caption{Blocks variant for BT-LSTM. ``N'' denotes the CP rank $N$. It's obvious that with additional blocks, the better accuracy is obtained.}
    \end{figure*}

    \begin{figure*}[h]
        \centering
        \subfigure[][Training Loss]{\includegraphics[height=0.14\columnwidth]{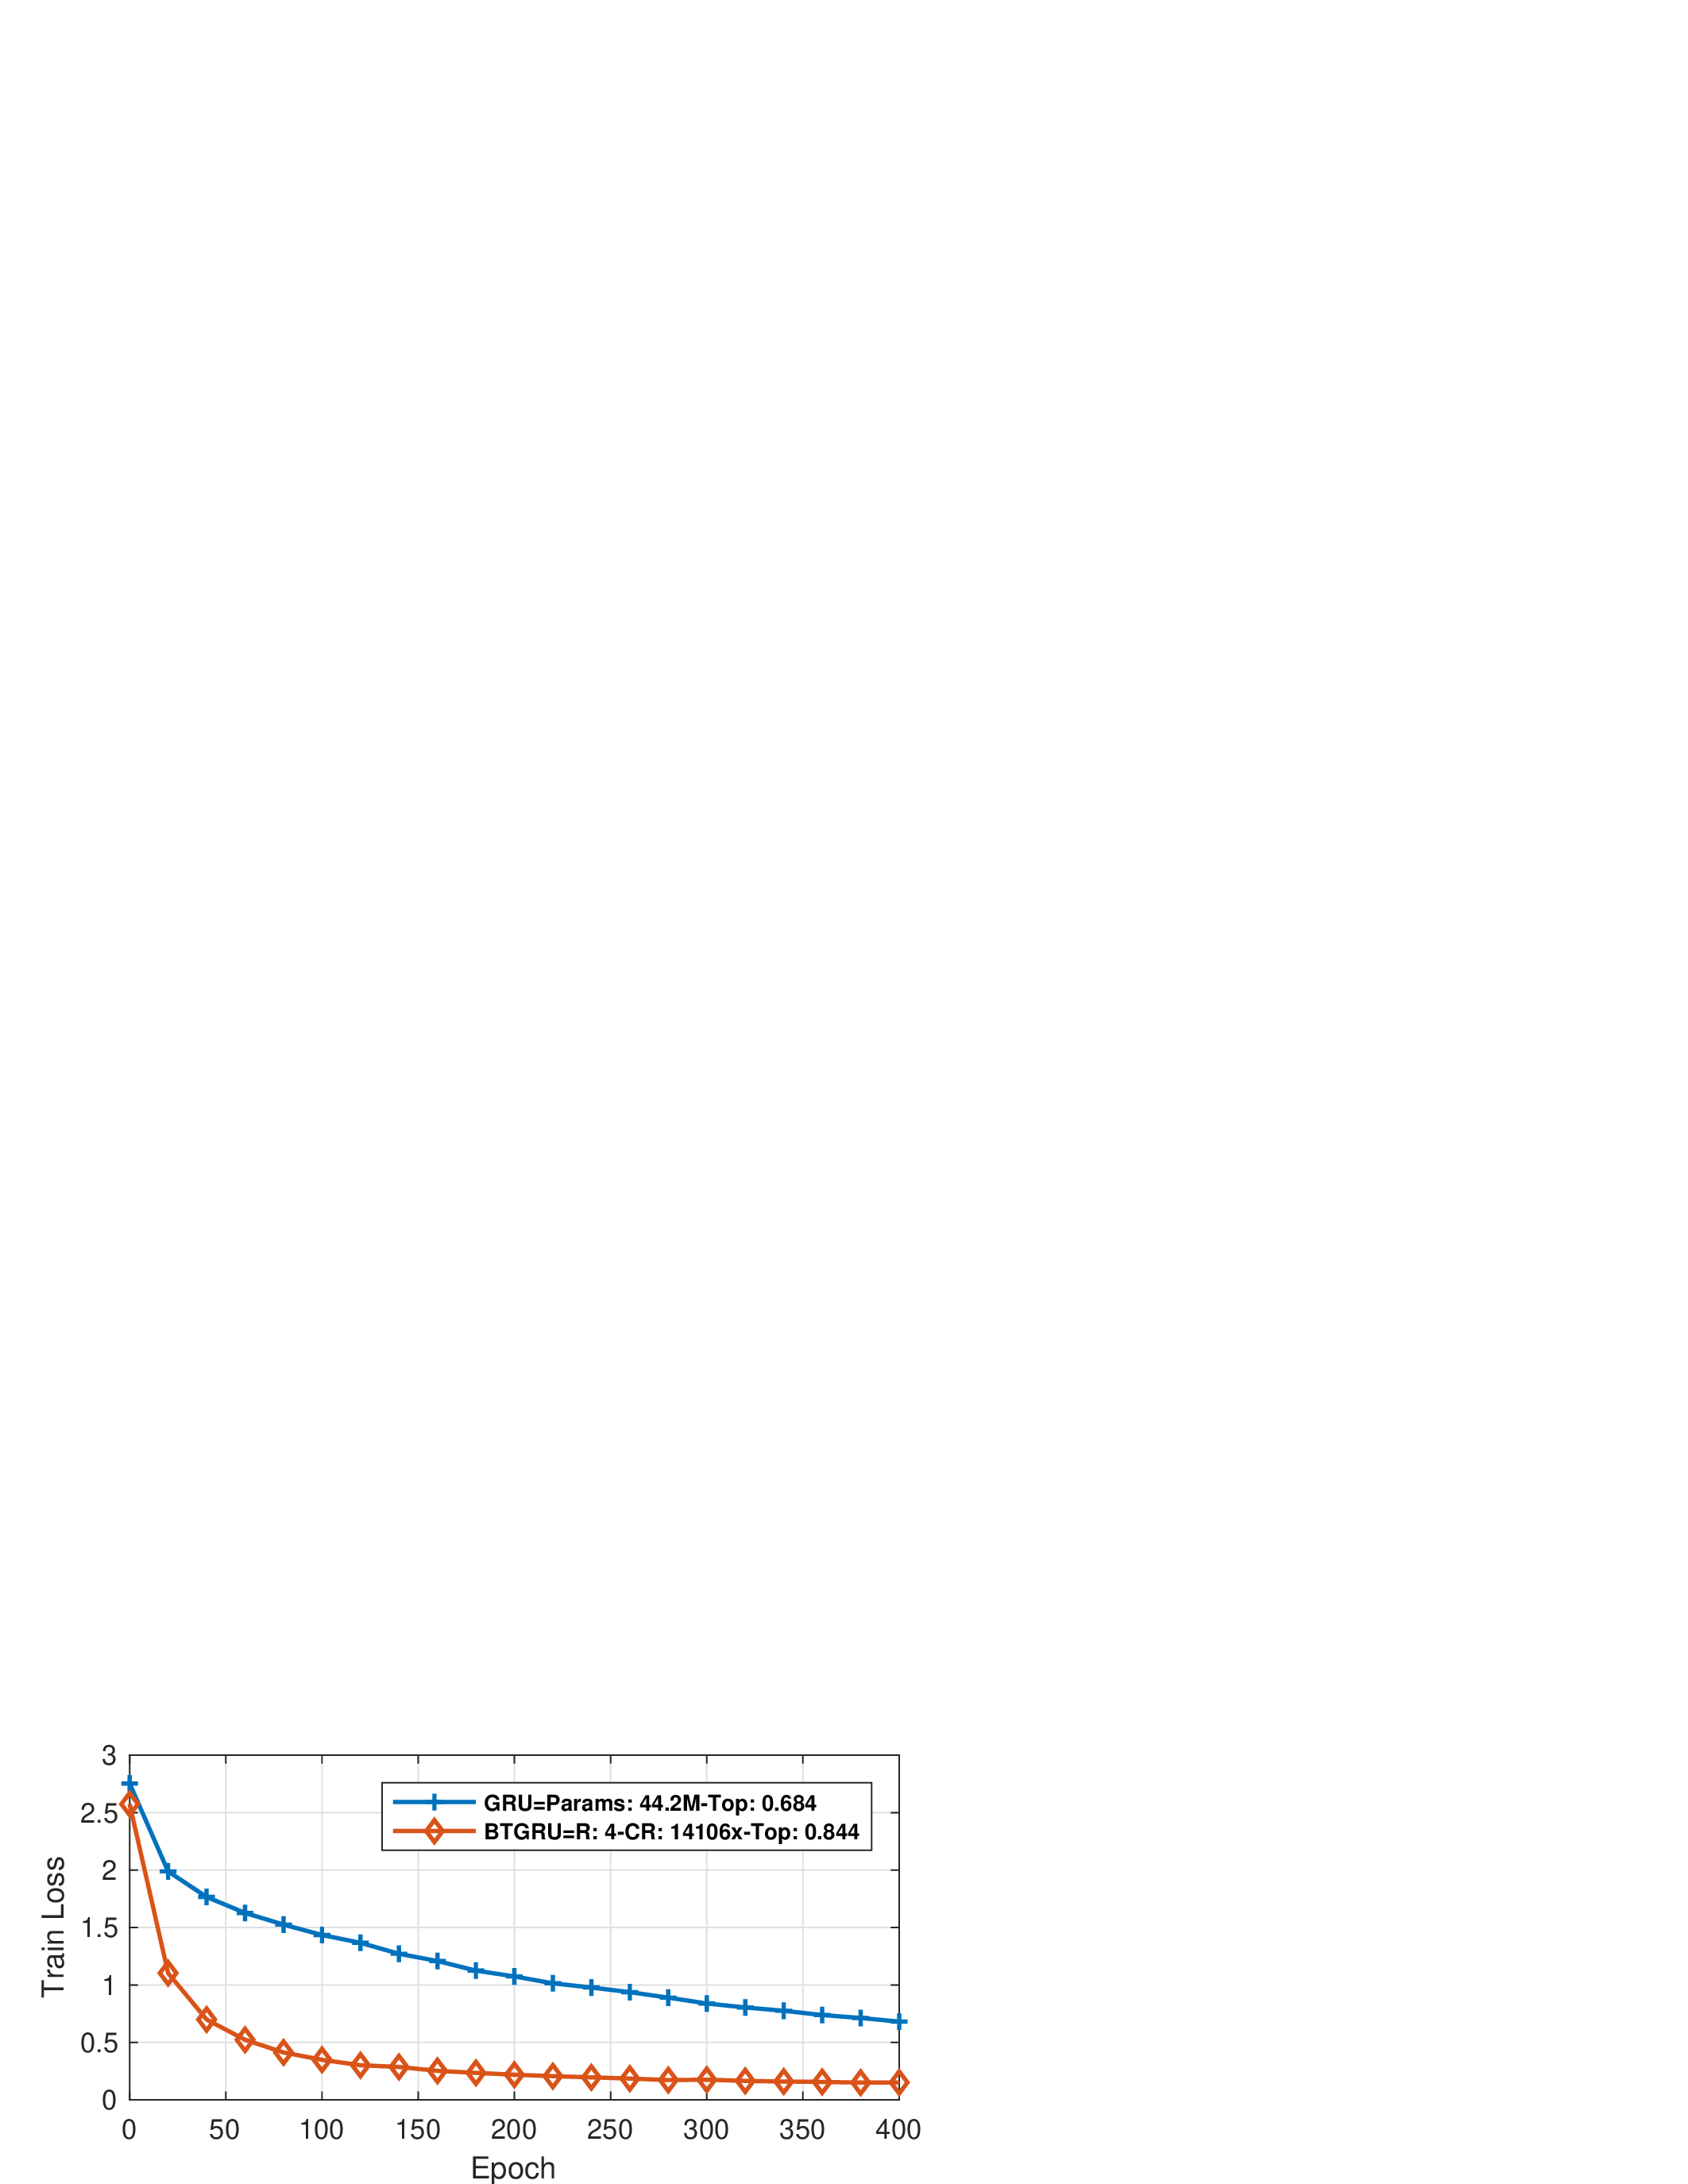}} \quad
        \subfigure[][Training Accuracy]{\includegraphics[height=0.14\columnwidth]{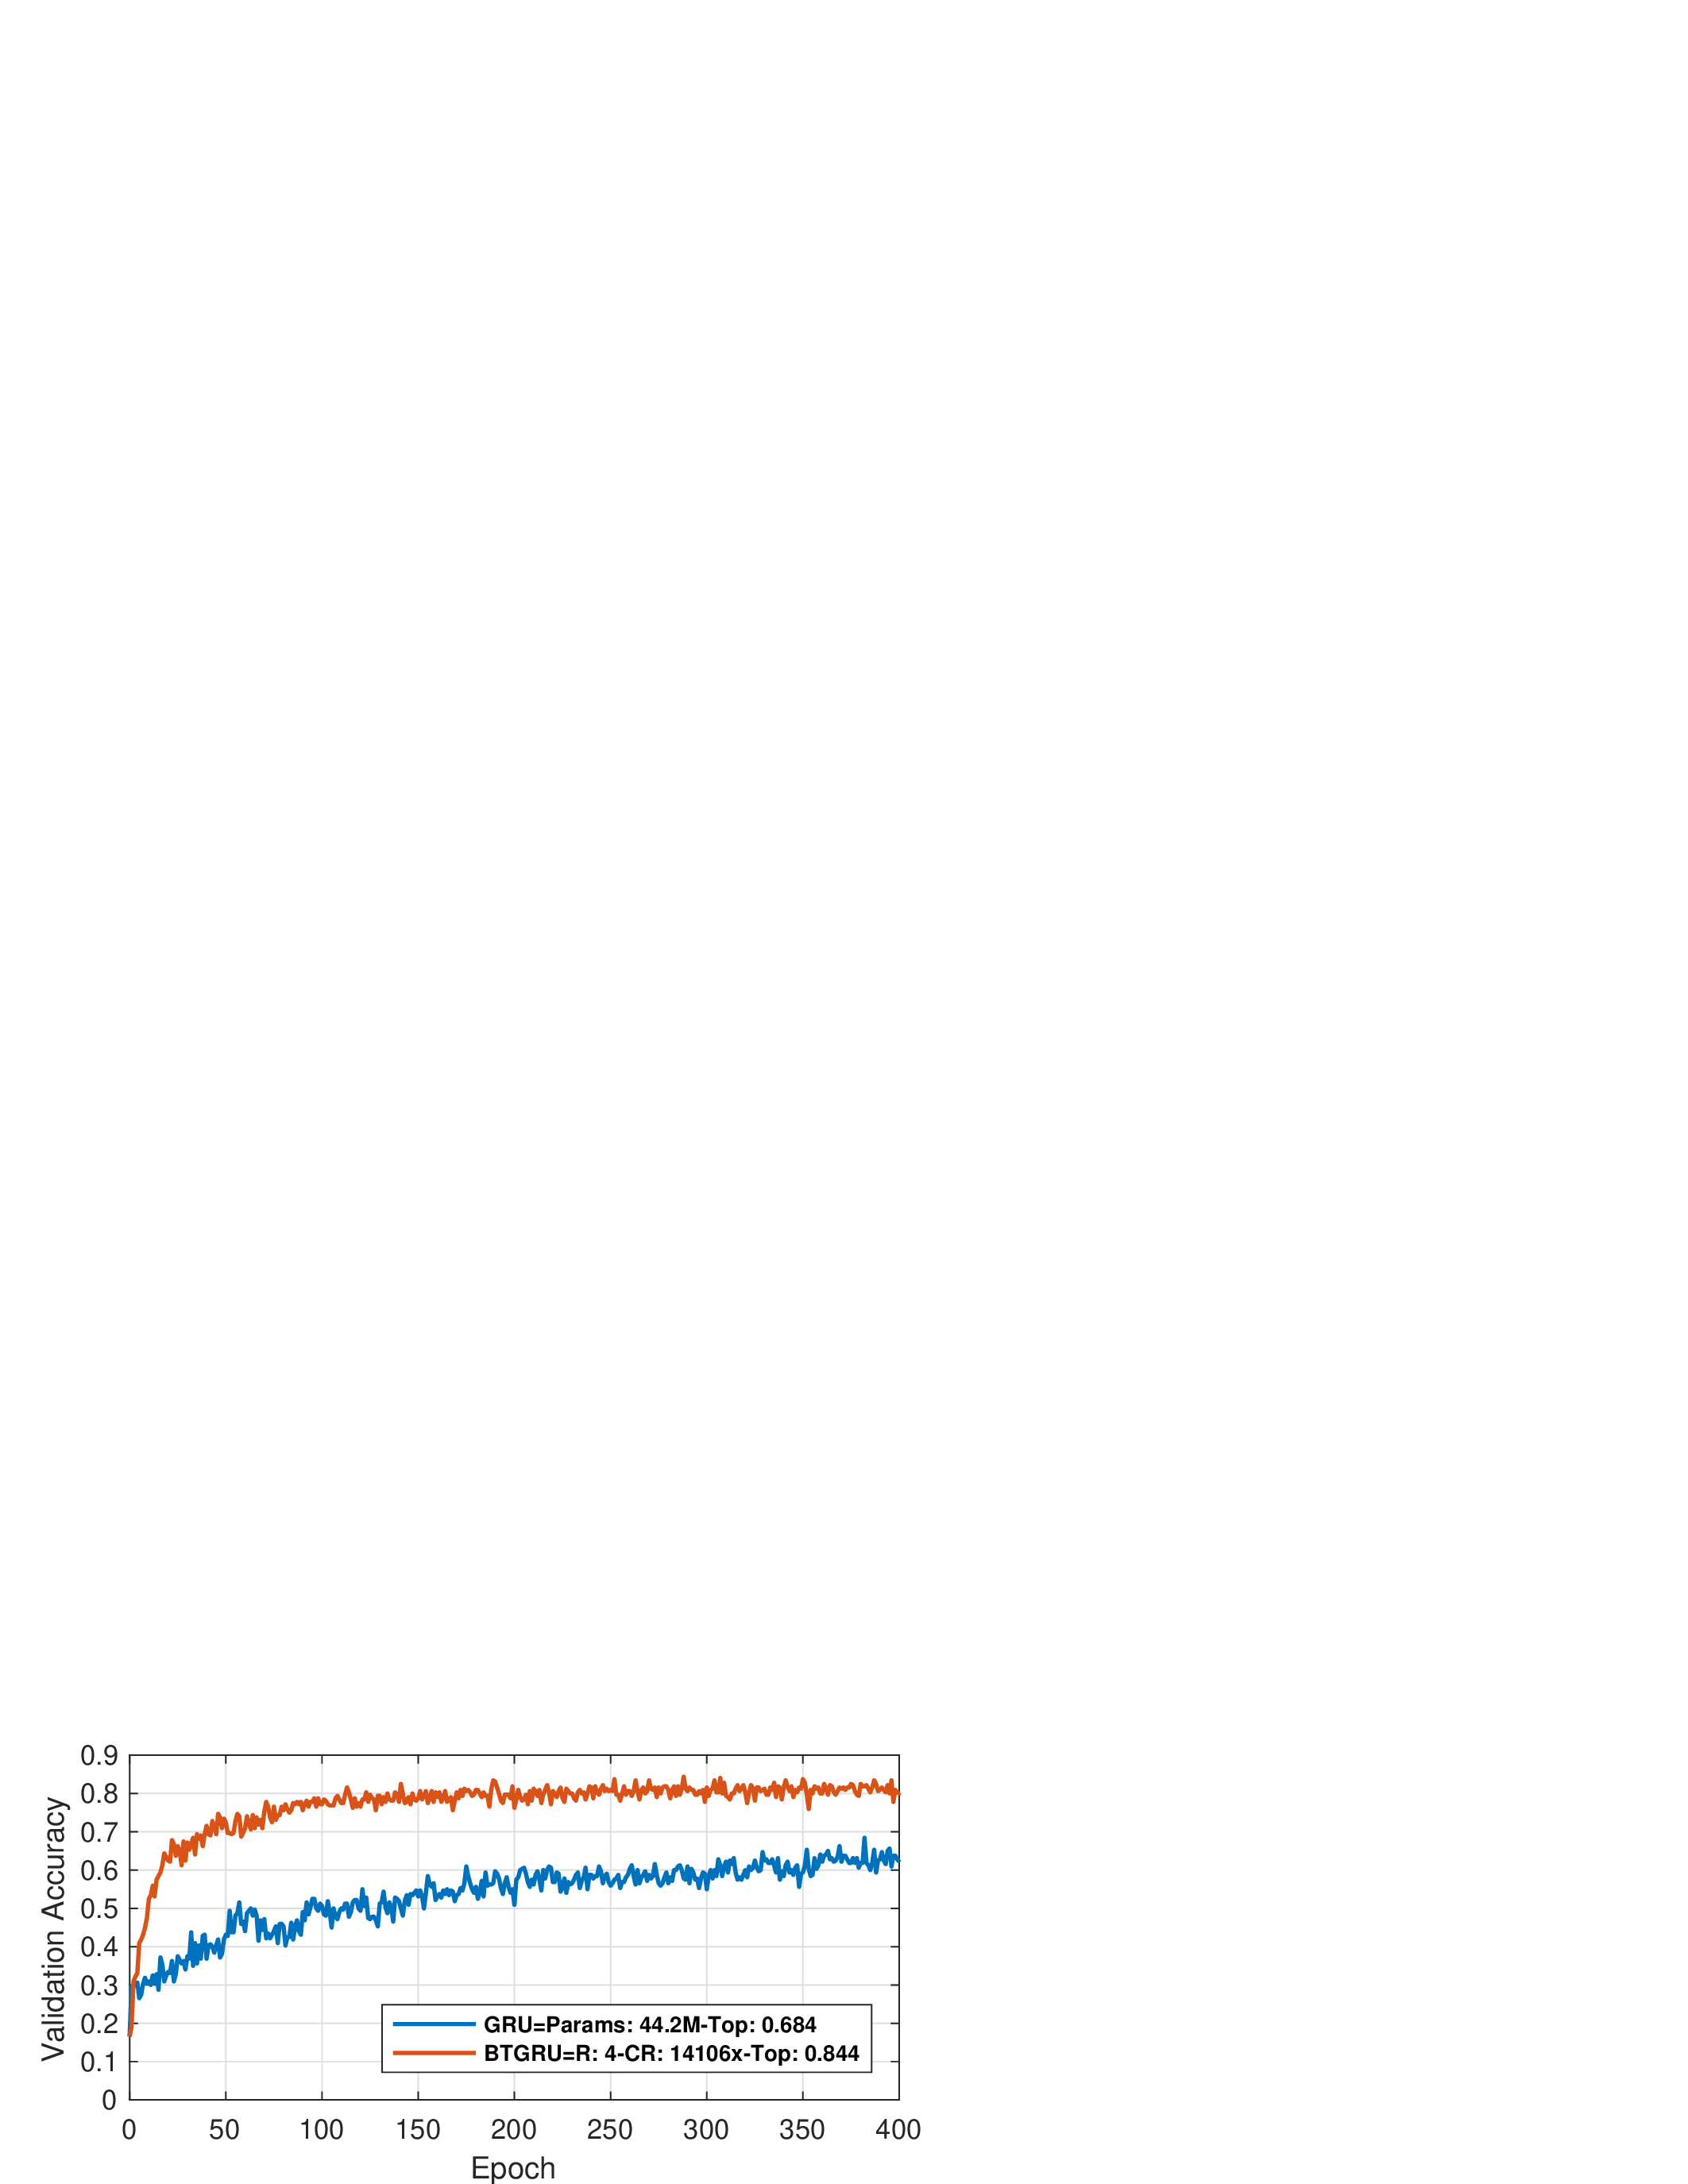}}
        \caption{BT-GRU test case. ``N'' is set to 2. The validation accuracies are 0.684 and 0.844 for GRU and BT-GRU respectively. In this test case, we show that our method can also be applied to other RNN structures and obtain better performance.}
    \end{figure*}

\subsection*{2. Numeric results of DRAW}
\begin{table}[h]
    \begin{center}
    \begin{tabular}{l|c|c}
    \hline
    Method & \#Params & Loss \\
    \hline\hline
    LSTM  & 1867776 & 94.24  \\
    BT-LSTM d=4,R=4 & 1184 & 93.38  \\
    TT-LSTM d=4,R=4 & 1264 & 97.75 \\
    % BT-LSTM d=2,R=2 & 6404 & 113.41 \\
    % TT-LSTM d=2,R=2 & 6400 & 113.92 \\
    \hline
    \end{tabular}
    \end{center}
    \caption{Results in DRAW. The block size of BT-LSTM is set to 1. Loss denotes the sum of the reconstruction and latent losses. But since there was no better metric to evaluate the quality of generated images and the gap in the loss is minor, it's hard to figure out the difference in various models.}
    \label{tbl:draw}
\end{table}

\subsection*{2. Numeric results of MSCOCO}
\begin{table}[h]
    \begin{center}
    \begin{tabular}{l|c|c|c}
    \hline
    Method & \#Params & BLEU-4 & CIDEr \\
    \hline\hline
    LSTM  & 1048576 & 0.299 & 0.910  \\ % 512*512*4
    BT-LSTM N=2 & 2048 & 0.307 & 0.921  \\ %  ((4*8*4+4*4+4*4+8*4)*4+4^4)*2 = 2048
    TT-LSTM & 1152 & 0.291 & 0.892 \\ % (8*4*4*4+16*16+16*16+8*4*4) = 1152
    BT-LSTM N=1 & 1024 & 0.303 & 0.915  \\ %  ((4*8*4+4*4+4*4+8*4)*4+4^4) = 1024
    \hline
    \end{tabular}
    \end{center}
    \caption{MSCOCO numerical results. BT-LSTM and TT-LSTM are set in d=4 and R=4.}
    \label{tbl:mscoco}
\end{table}
